# Supplementary material for: Understanding and Tackling Scattering and Reflective Flare for Mobile Camera Systems
Source: arXiv:2307.14180 source file (2024-11-04)
Supplement: Supplementary file 1 [file appendix.tex]

\clearpage
\appendix
In this supplementary material, we provide more details about network training as well as more visual comparison between the real and synthetic dataset. We also provide more experimental results in the following section. 

\begin{figure*}
  \begin{tikzpicture}
        % First row
        \node[inner sep=0pt] (fig1) at (0,0) {\includegraphics[width=0.09\linewidth]{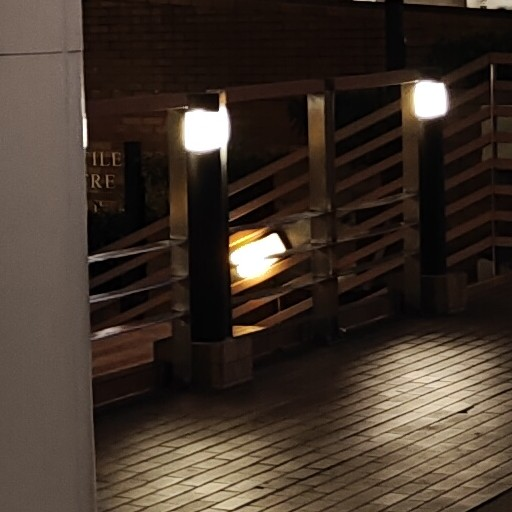}};
        \node[inner sep=0pt, right=0.05cm of fig1] (fig2) {\includegraphics[width=0.09\linewidth]{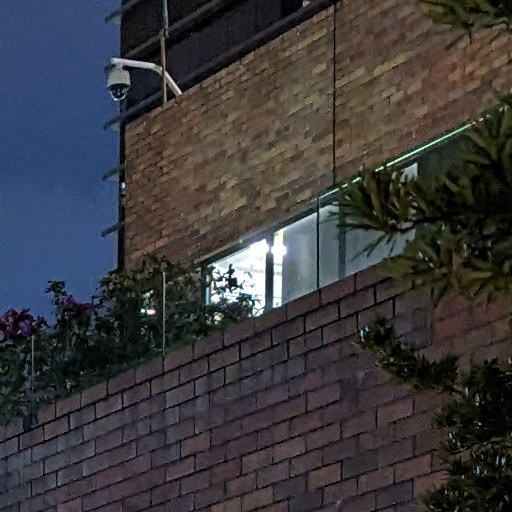}};
        \node[inner sep=0pt, right=0.05cm of fig2] (fig3) {\includegraphics[width=0.09\linewidth]{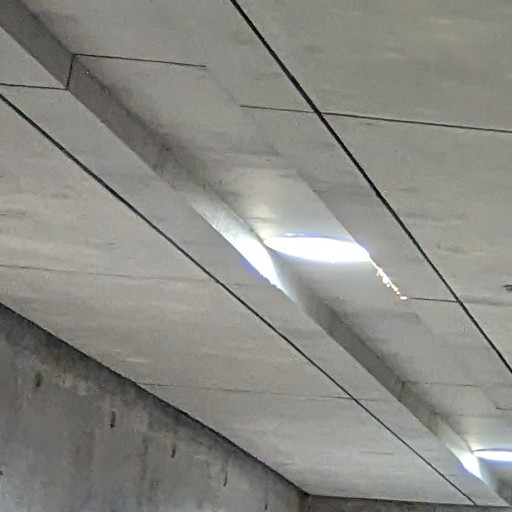}};
        \node[inner sep=0pt, right=0.05cm of fig3] (fig4) {\includegraphics[width=0.09\linewidth]{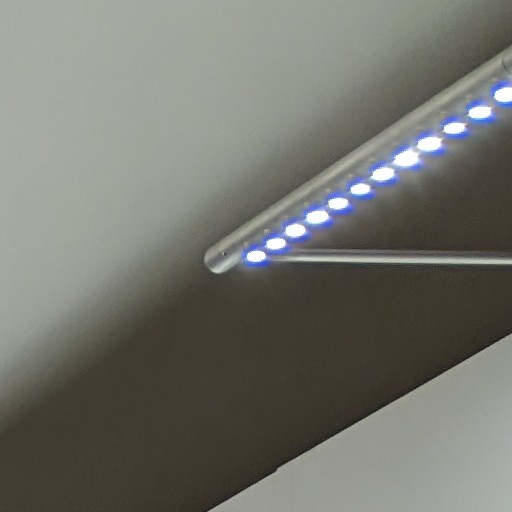}};
        \node[inner sep=0pt, right=0.05cm of fig4] (fig5) {\includegraphics[width=0.09\linewidth]{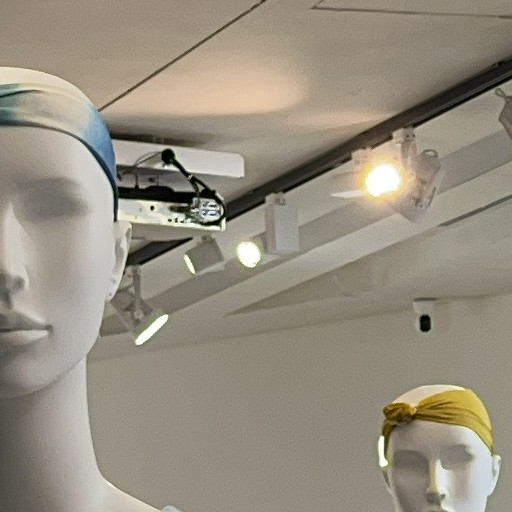}};
        \node[inner sep=0pt, right=0.15cm of fig5] (fig6) {\includegraphics[width=0.09\linewidth]{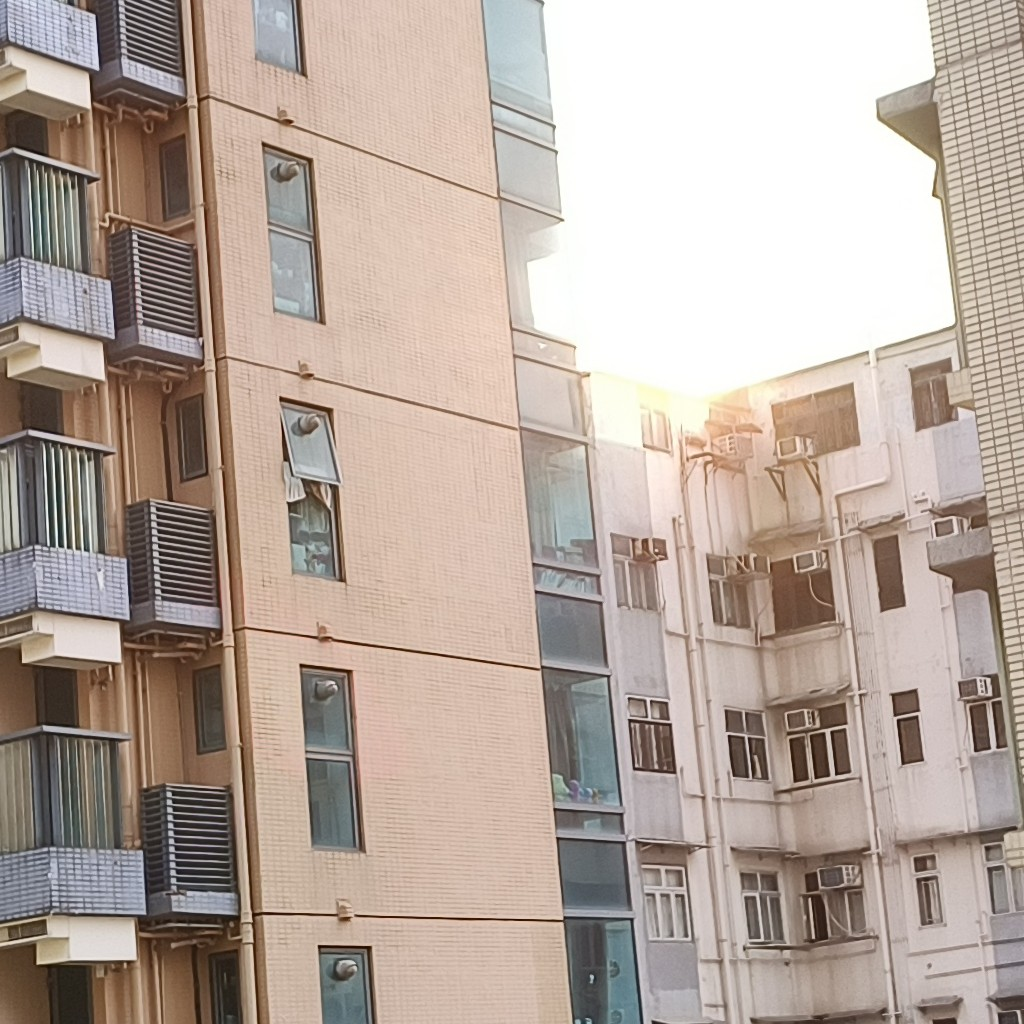}};
        \node[inner sep=0pt, right=0.05cm of fig6] (fig7) {\includegraphics[width=0.09\linewidth]{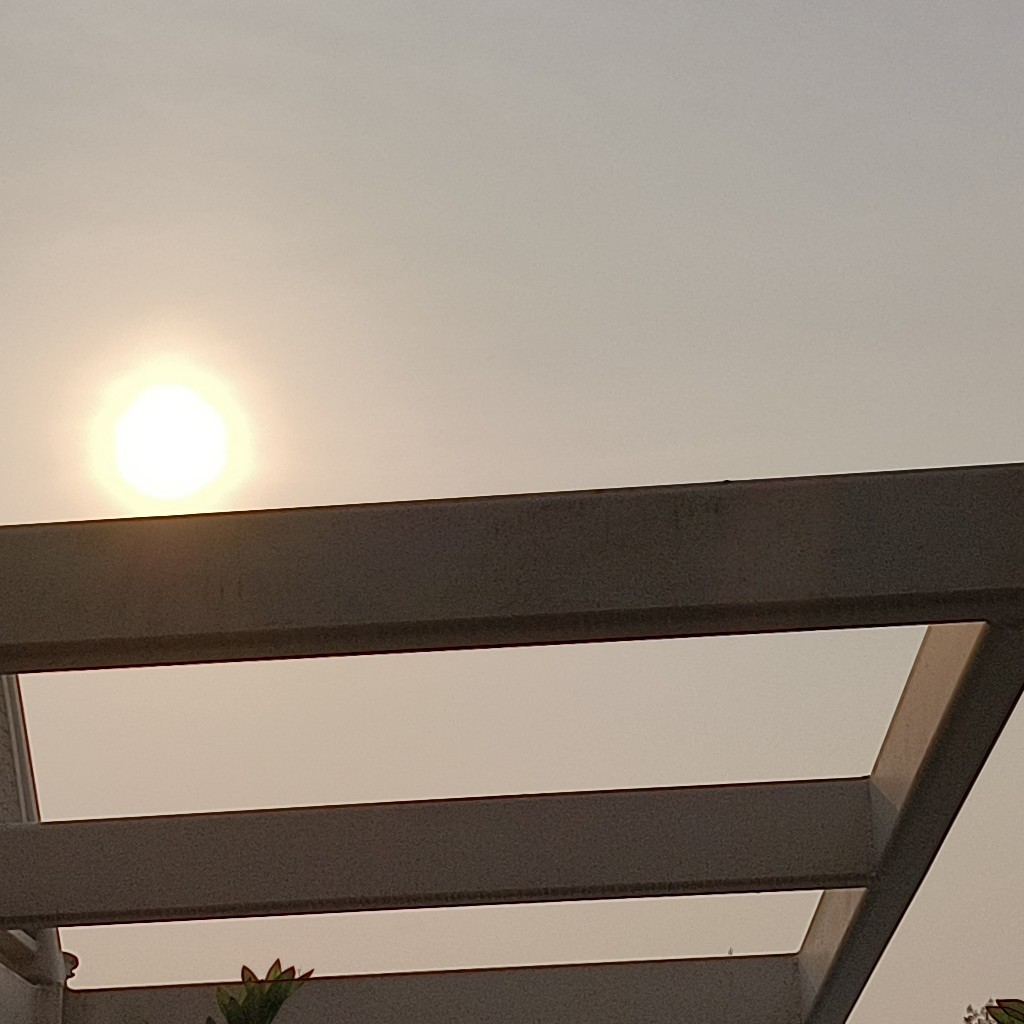}};
        \node[inner sep=0pt, right=0.05cm of fig7] (fig8) {\includegraphics[width=0.09\linewidth]{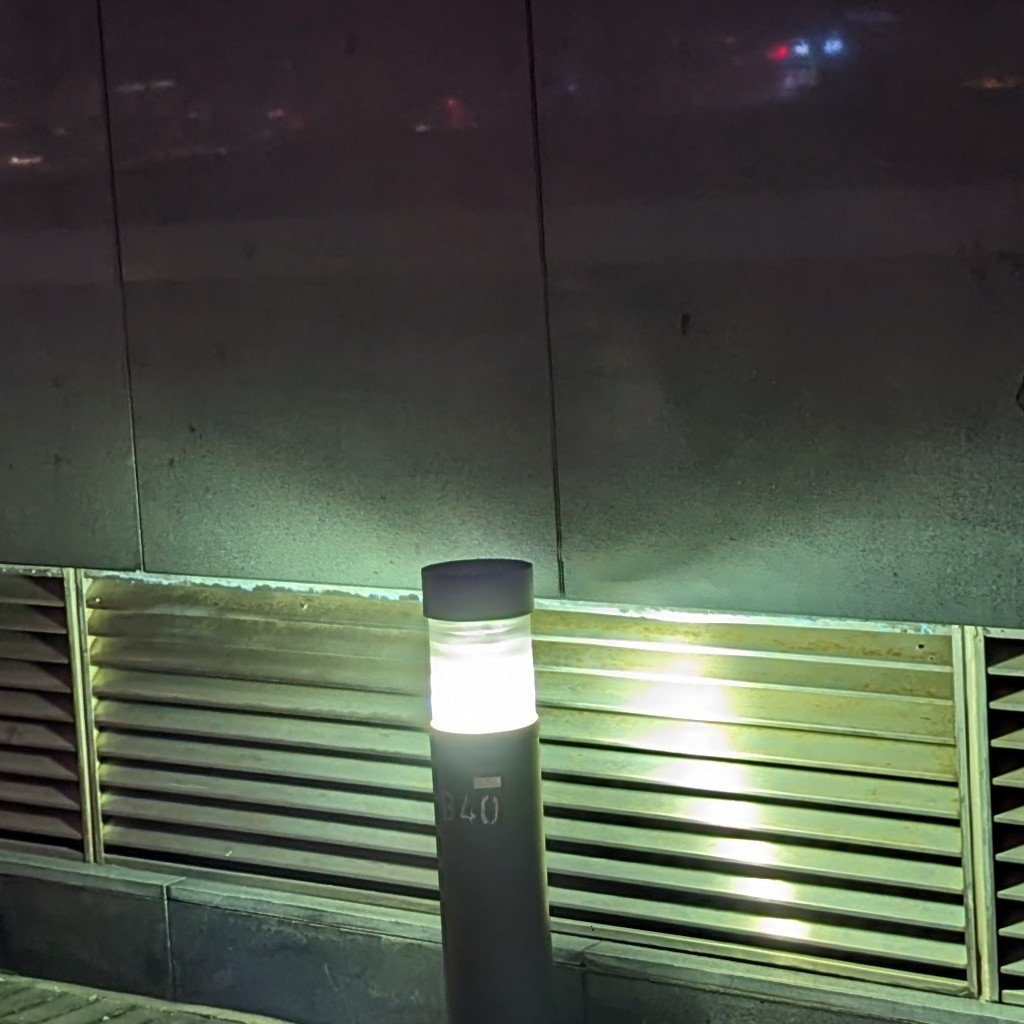}};
         \node[inner sep=0pt, right=0.05cm of fig8] (fig9) {\includegraphics[width=0.09\linewidth]{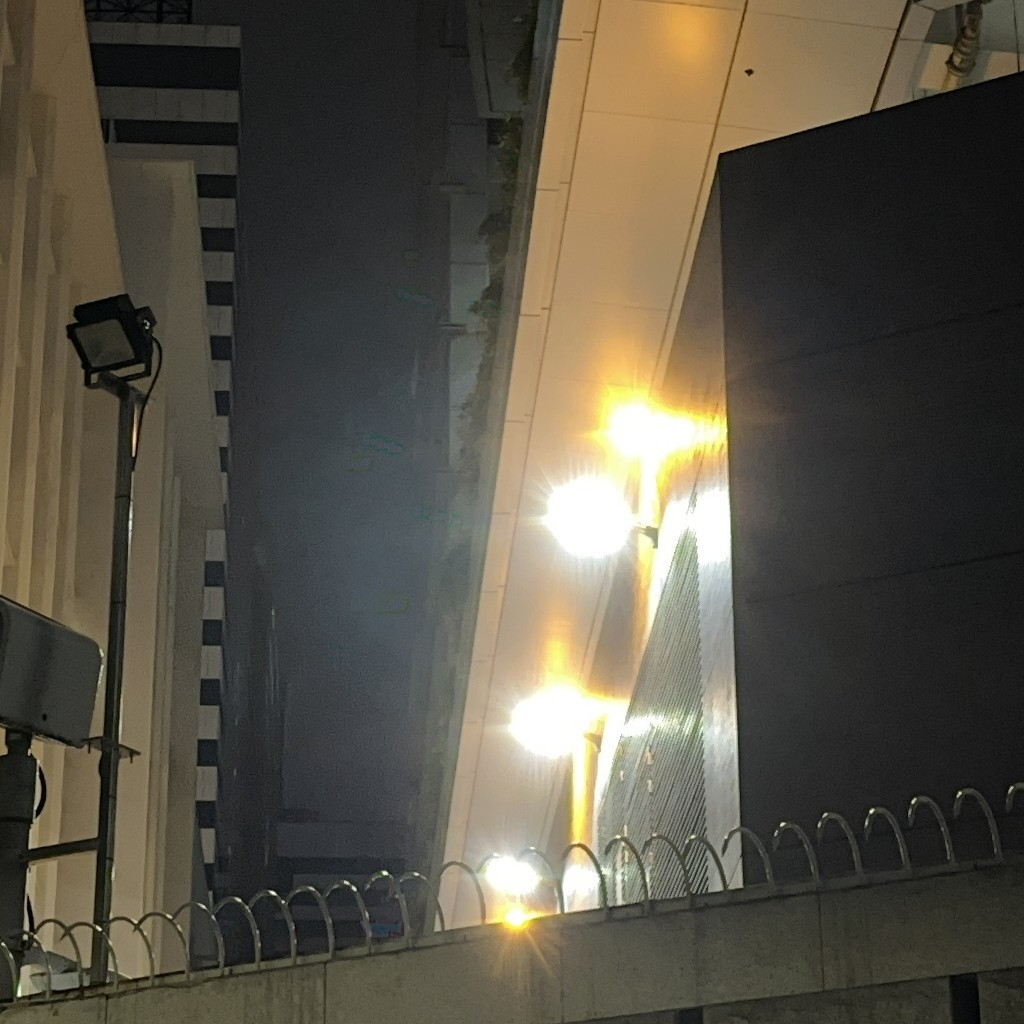}};
          \node[inner sep=0pt, right=0.05cm of fig9] (fig10) {\includegraphics[width=0.09\linewidth]{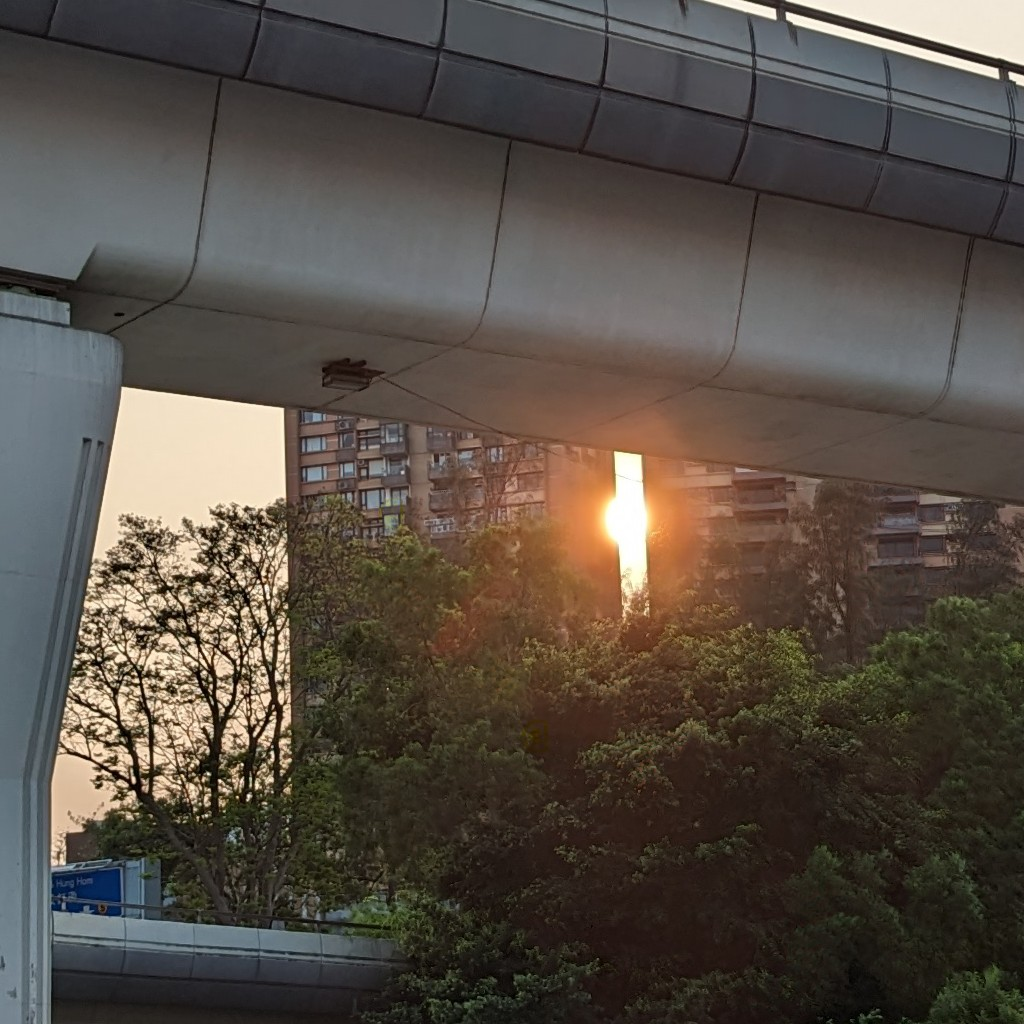}};
           % First row
         \node[inner sep=0pt, below=0.05cm of fig1] (fig11){\includegraphics[width=0.09\linewidth]{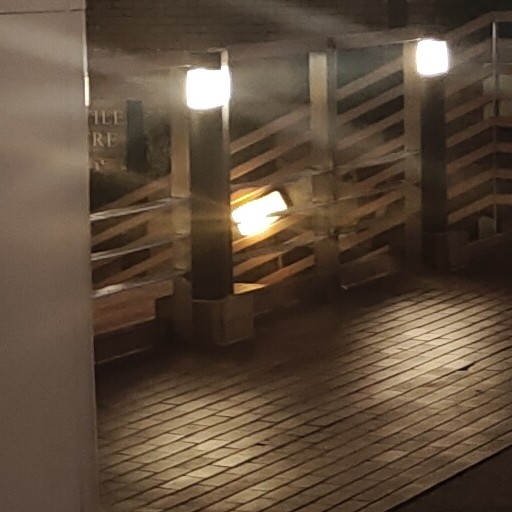}};
        \node[inner sep=0pt, right=0.05cm of fig11] (fig12) {\includegraphics[width=0.09\linewidth]{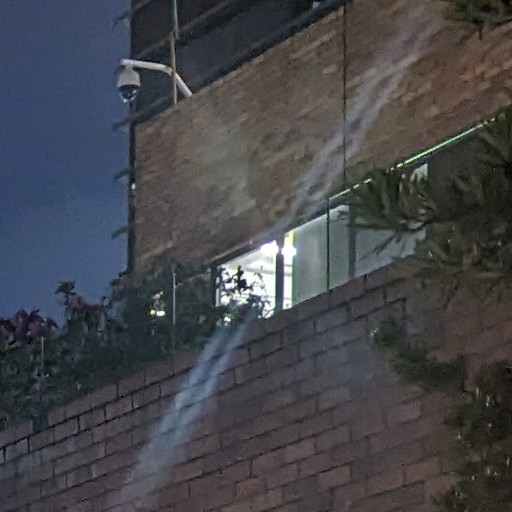}};
        \node[inner sep=0pt, right=0.05cm of fig12] (fig13) {\includegraphics[width=0.09\linewidth]{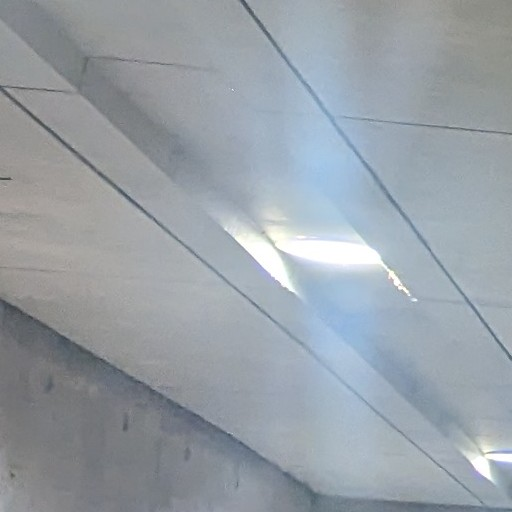}};
        \node[inner sep=0pt, right=0.05cm of fig13] (fig14) {\includegraphics[width=0.09\linewidth]{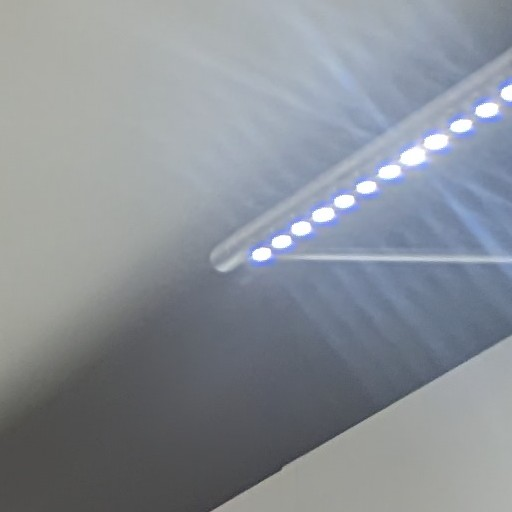}};
        \node[inner sep=0pt, right=0.05cm of fig14] (fig15) {\includegraphics[width=0.09\linewidth]{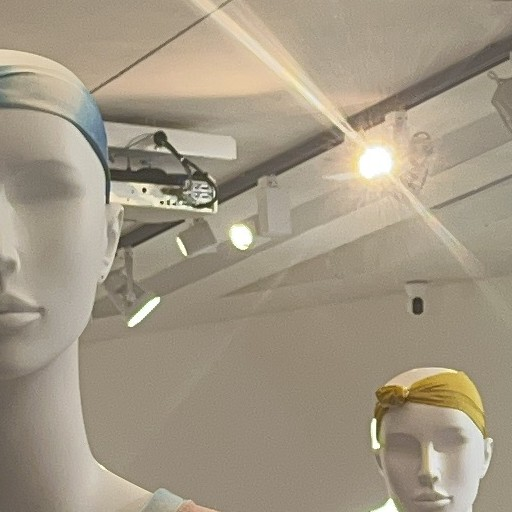}};
         \node[inner sep=0pt, right=0.15cm of fig15] (fig16) {\includegraphics[width=0.09\linewidth]{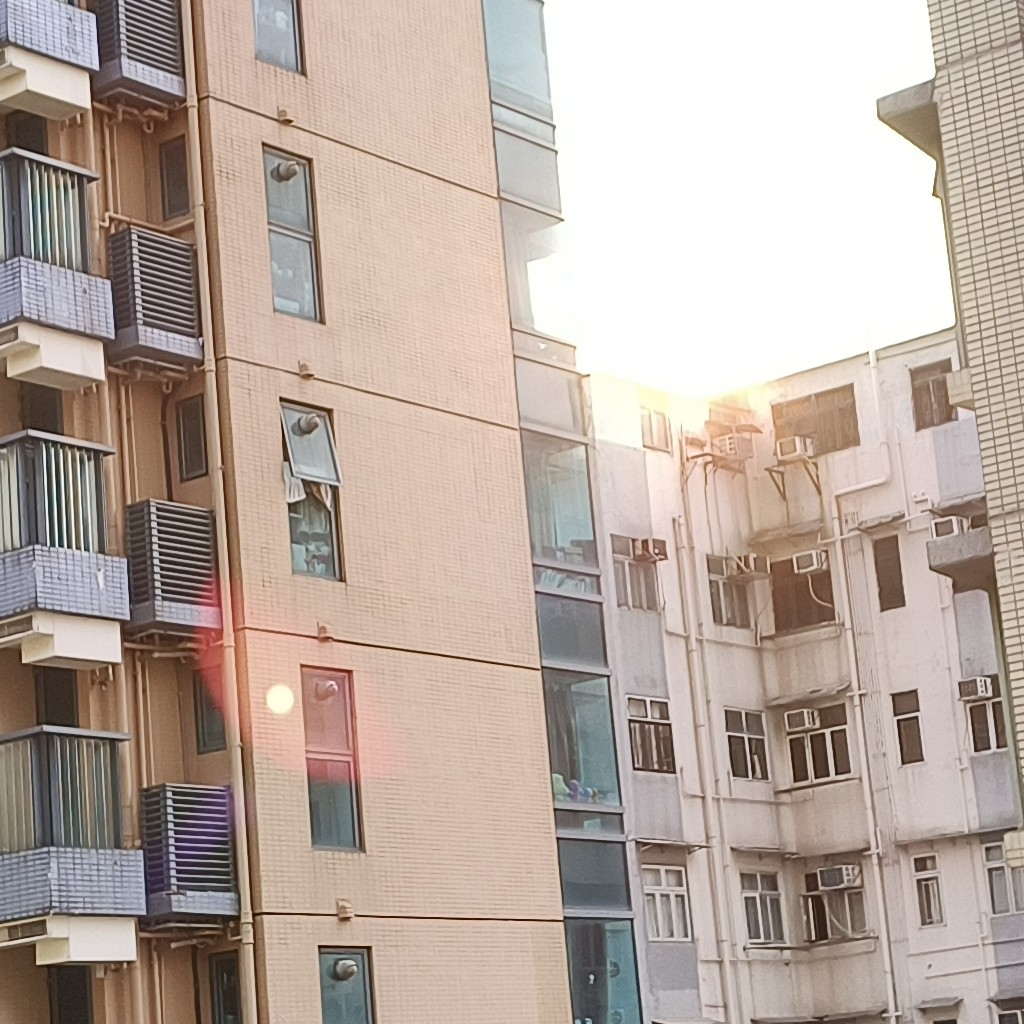}};
        \node[inner sep=0pt, right=0.05cm of fig16] (fig17) {\includegraphics[width=0.09\linewidth]{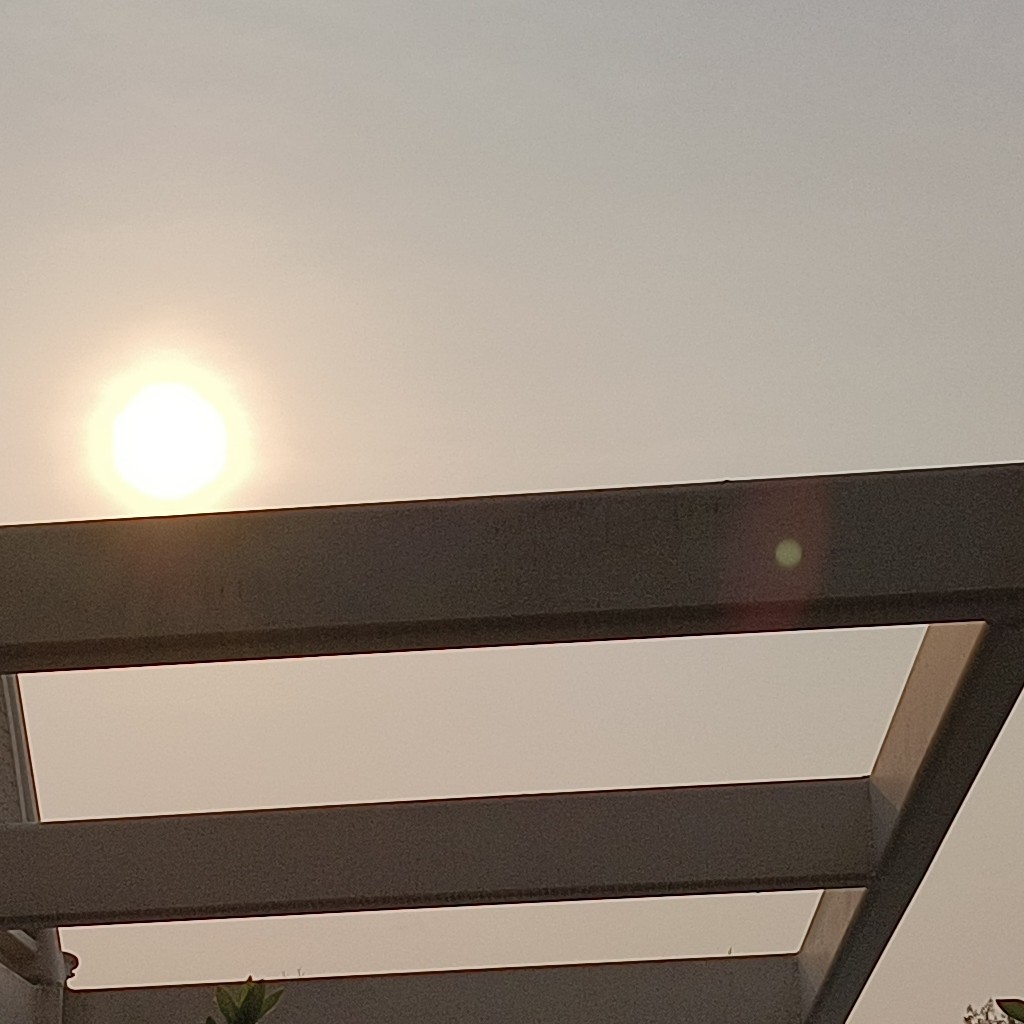}};
        \node[inner sep=0pt, right=0.05cm of fig17] (fig18) {\includegraphics[width=0.09\linewidth]{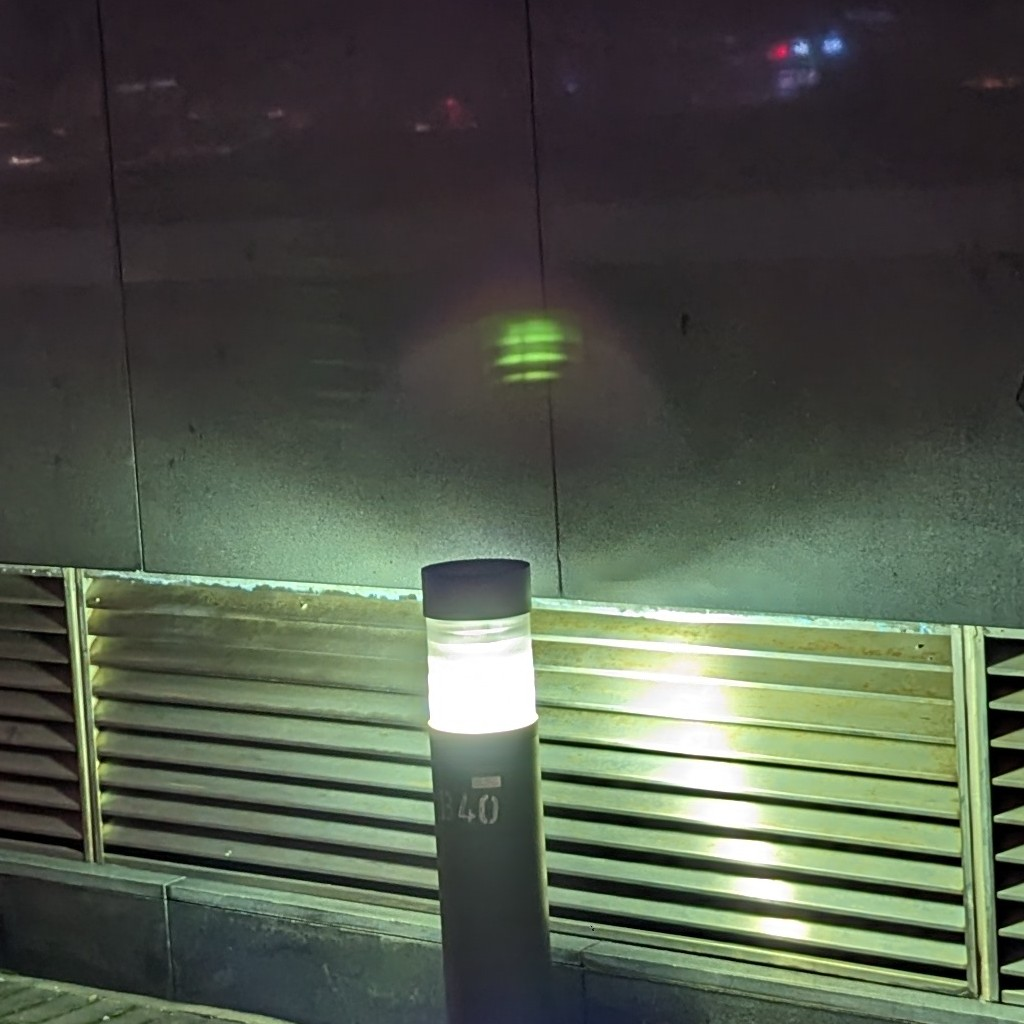}};
         \node[inner sep=0pt, right=0.05cm of fig18] (fig19) {\includegraphics[width=0.09\linewidth]{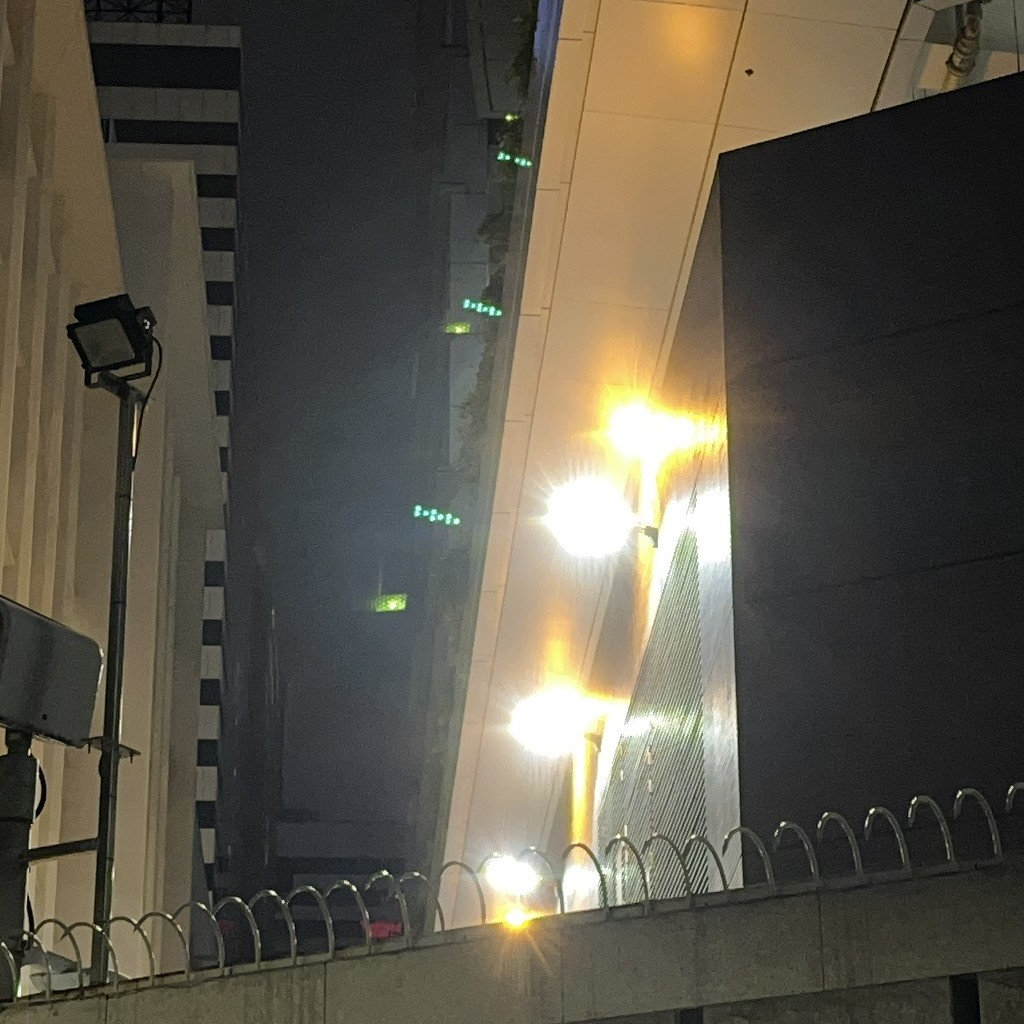}};
          \node[inner sep=0pt, right=0.05cm of fig19] (fig20) {\includegraphics[width=0.09\linewidth]{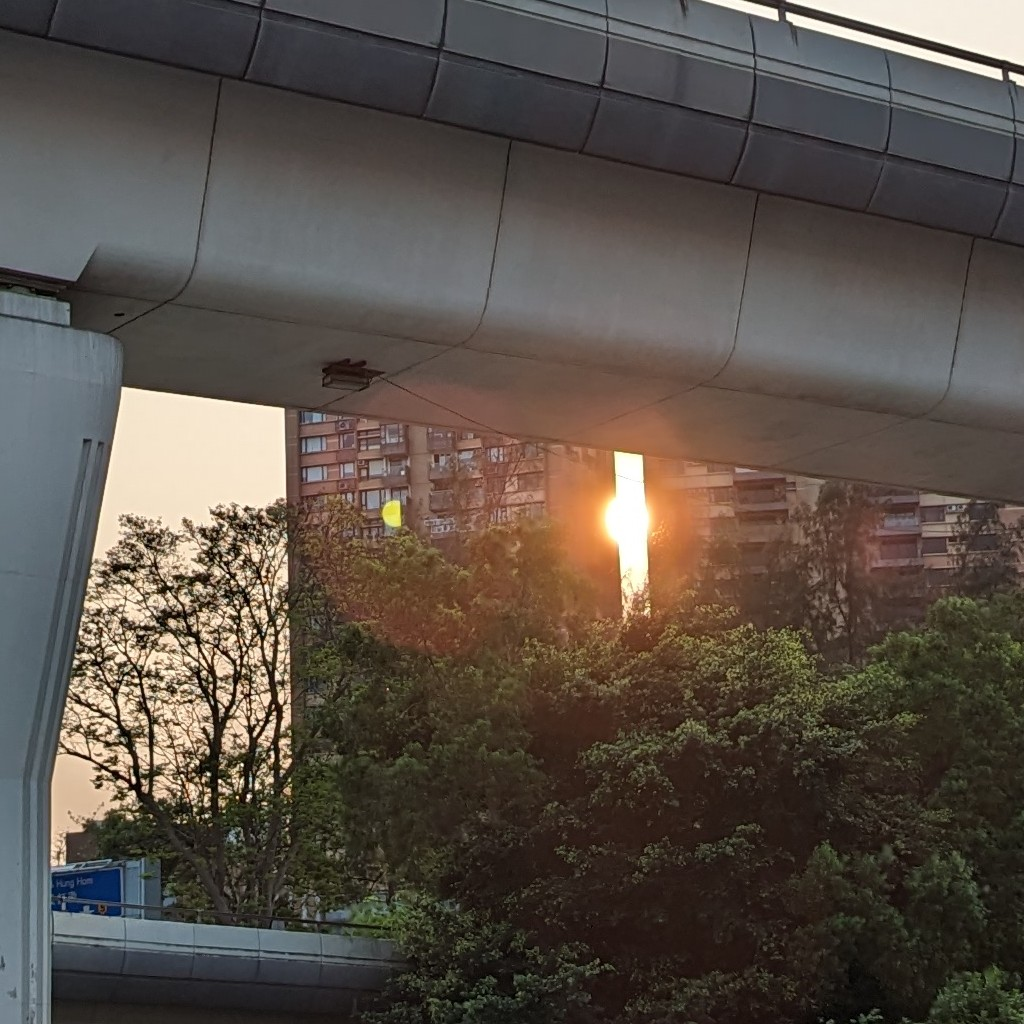}};
        % Second row
        \node[inner sep=0pt, below=0.05cm of fig11] (fig21) {\includegraphics[width=0.09\linewidth]{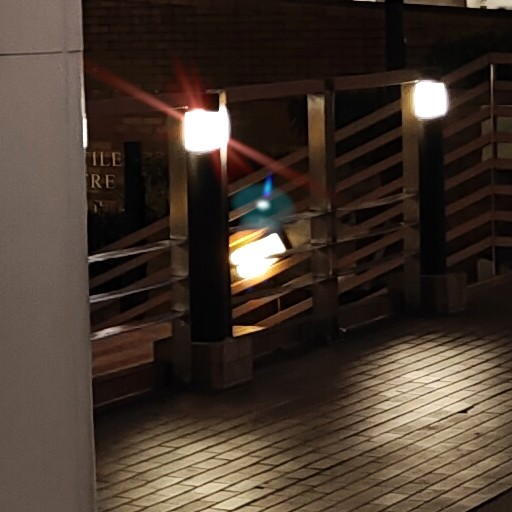}};
        \node[inner sep=0pt, right=0.05cm of fig21] (fig22) {\includegraphics[width=0.09\linewidth]{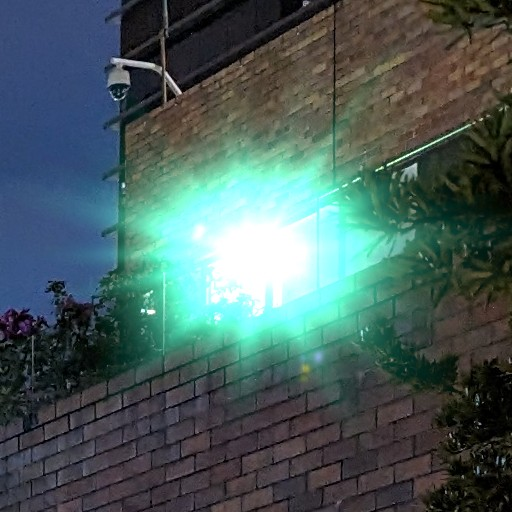}};
        \node[inner sep=0pt, right=0.05cm of fig22] (fig23) {\includegraphics[width=0.09\linewidth]{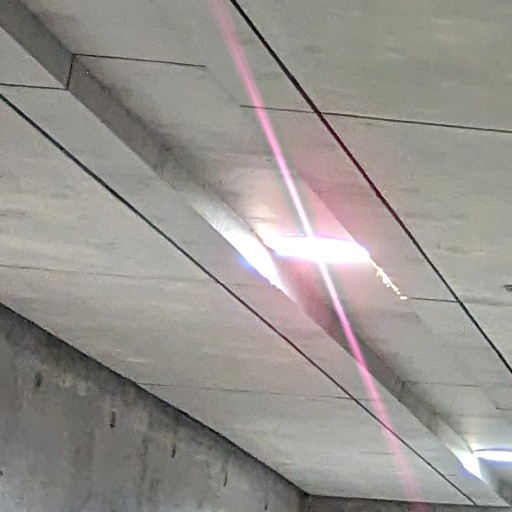}};
        \node[inner sep=0pt, right=0.05cm of fig23] (fig24) {\includegraphics[width=0.09\linewidth]{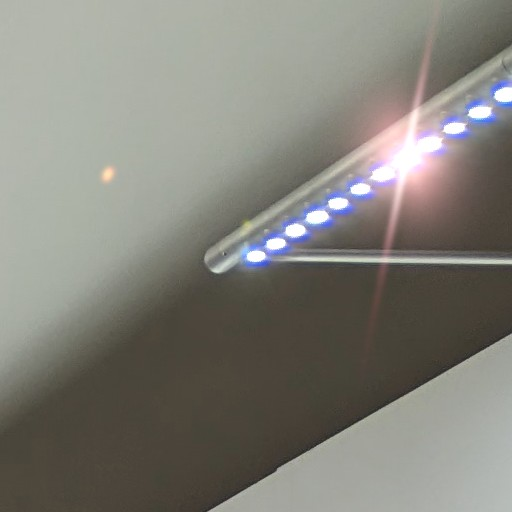}};
        \node[inner sep=0pt, right=0.05cm of fig24] (fig25) {\includegraphics[width=0.09\linewidth]{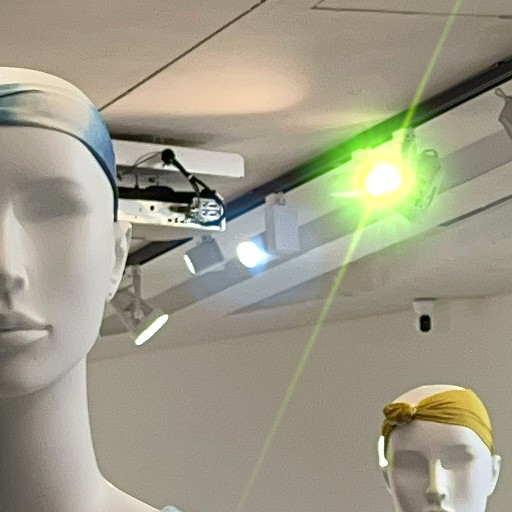}};
        \node[inner sep=0pt, right=0.15cm of fig25] (fig26) {\includegraphics[width=0.09\linewidth]{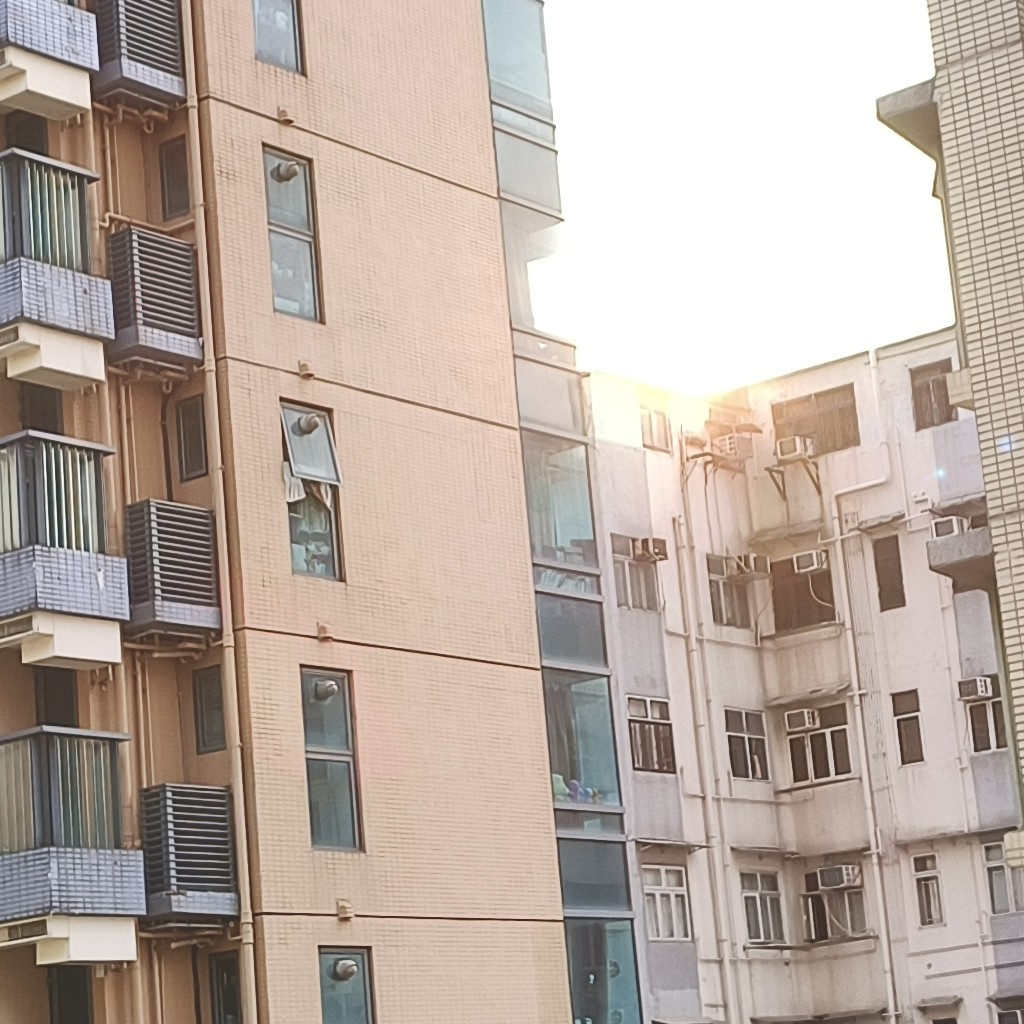}};
        \node[inner sep=0pt, right=0.05cm of fig26] (fig27) {\includegraphics[width=0.09\linewidth]{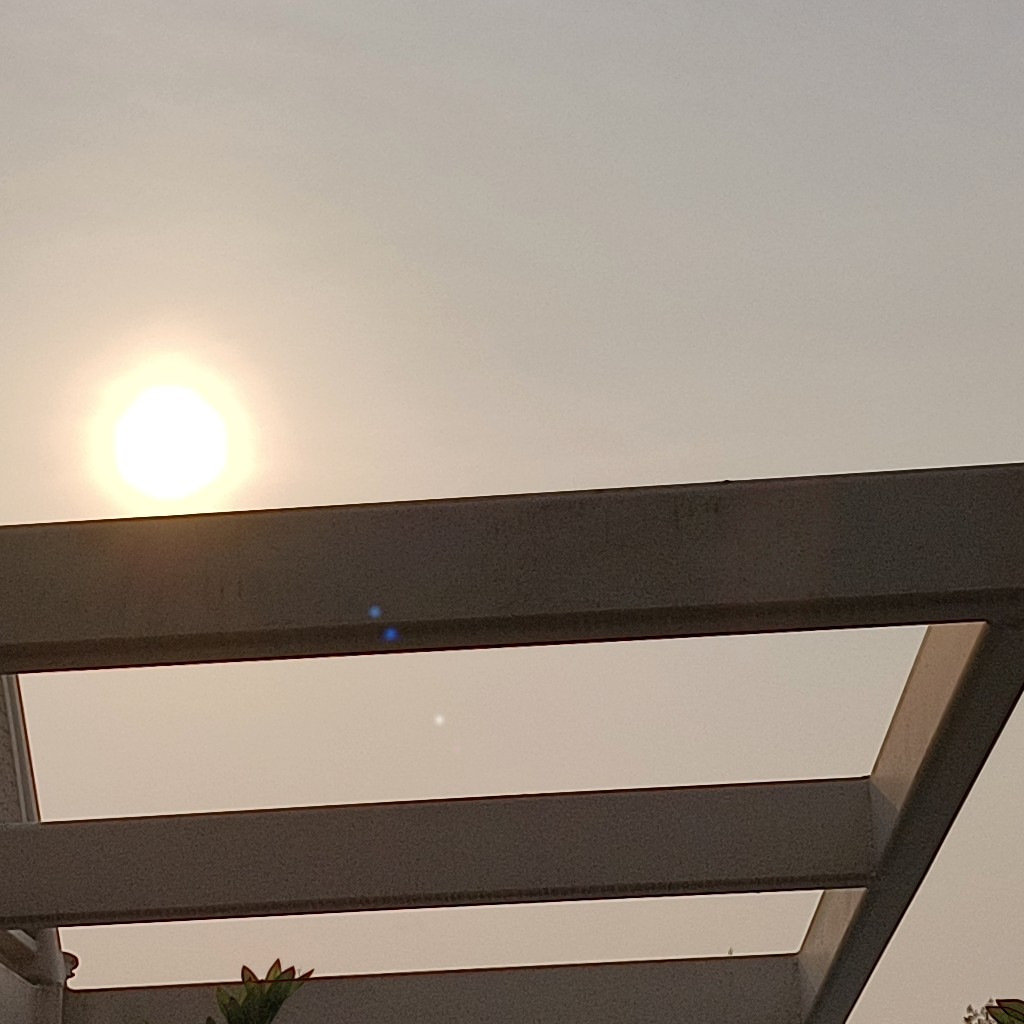}};
        \node[inner sep=0pt, right=0.05cm of fig27] (fig28) {\includegraphics[width=0.09\linewidth]{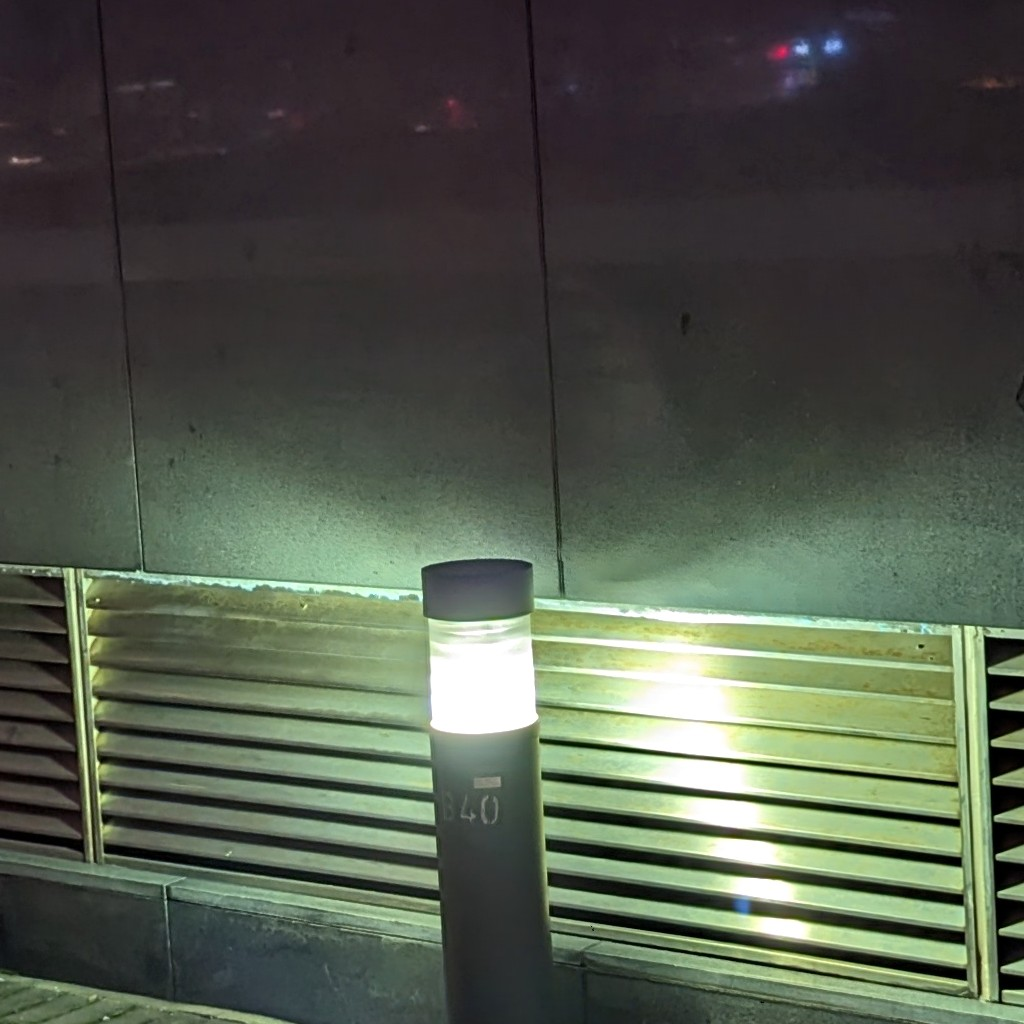}};
         \node[inner sep=0pt, right=0.05cm of fig28] (fig29) {\includegraphics[width=0.09\linewidth]{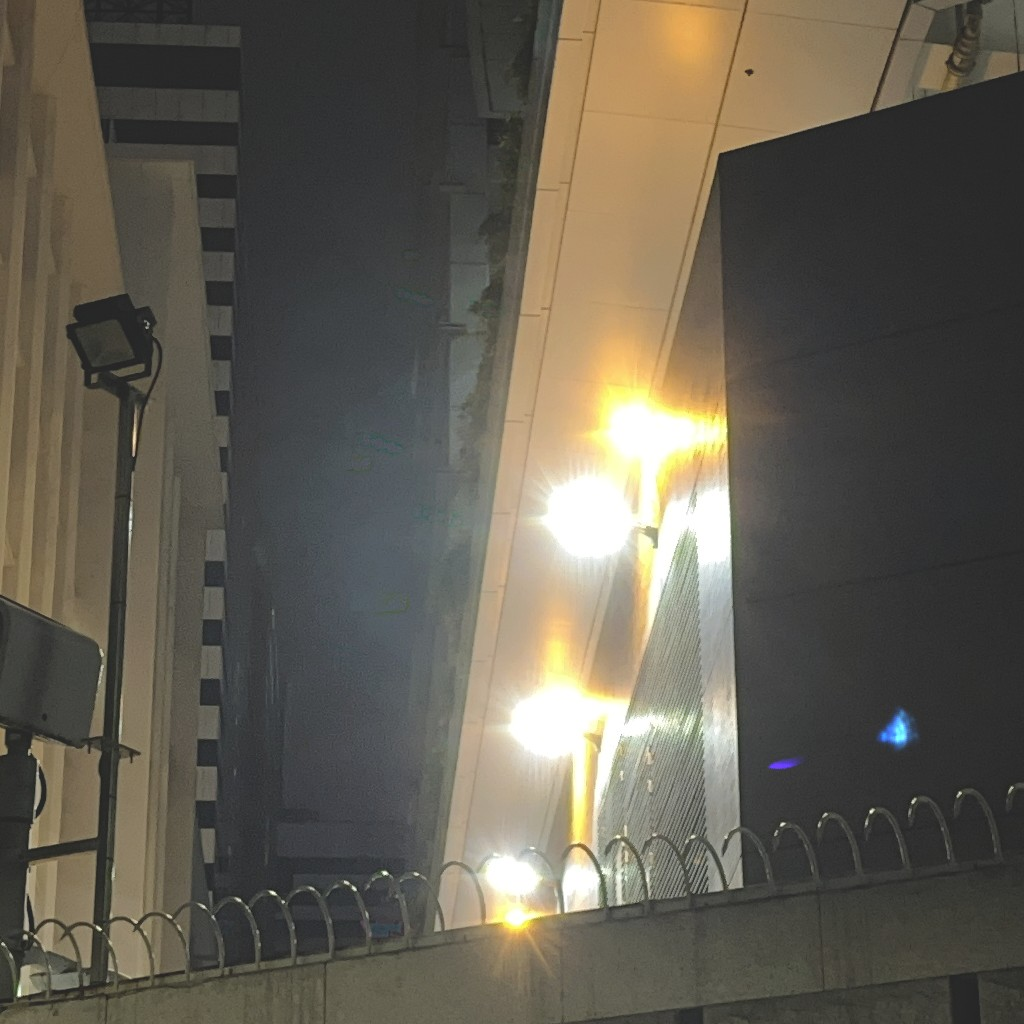}};
          \node[inner sep=0pt, right=0.05cm of fig29] (fig30) {\includegraphics[width=0.09\linewidth]{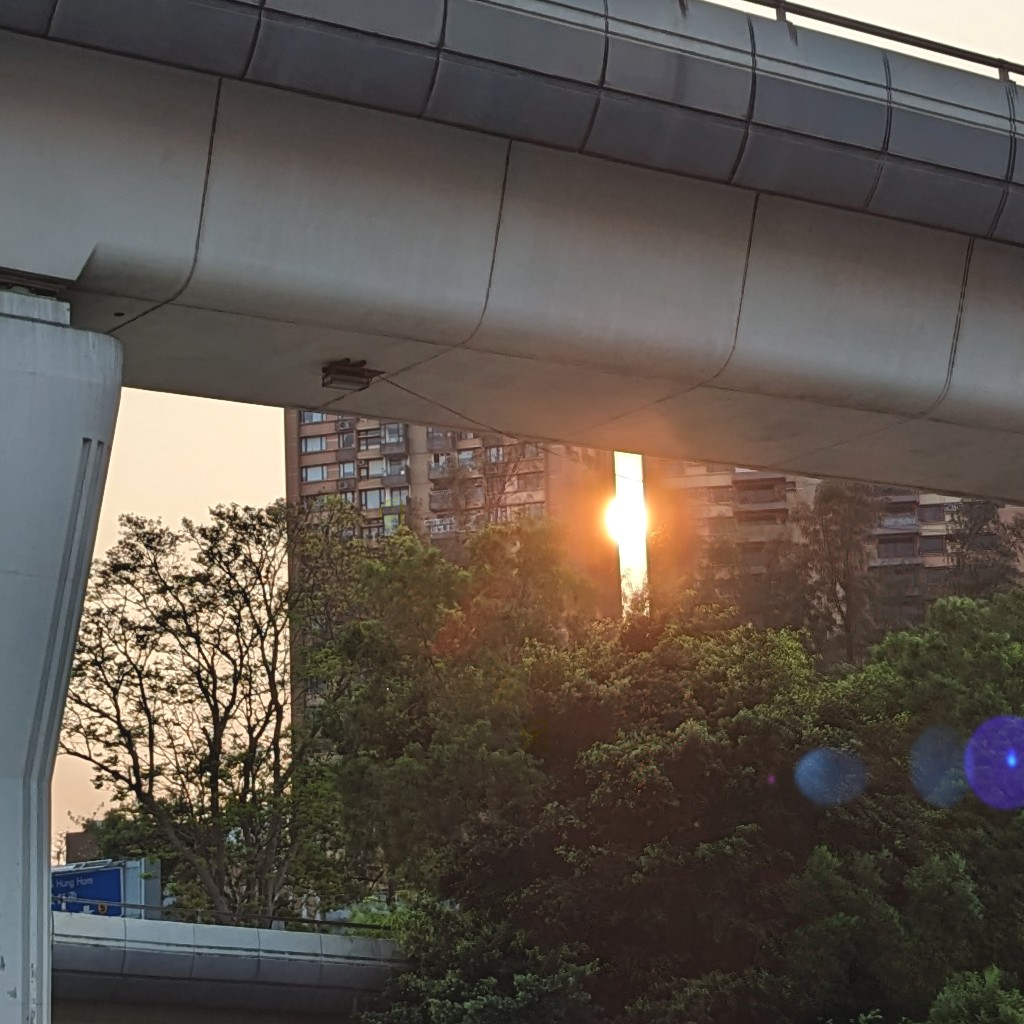}};
          
 % --------------
          \node[inner sep=0pt, below=0.15cm of fig21] (fig31)  {\includegraphics[width=0.09\linewidth]{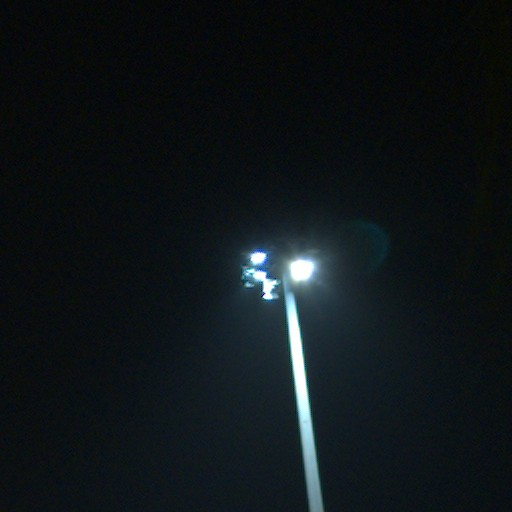}};
        \node[inner sep=0pt, right=0.05cm of fig31] (fig32) {\includegraphics[width=0.09\linewidth]{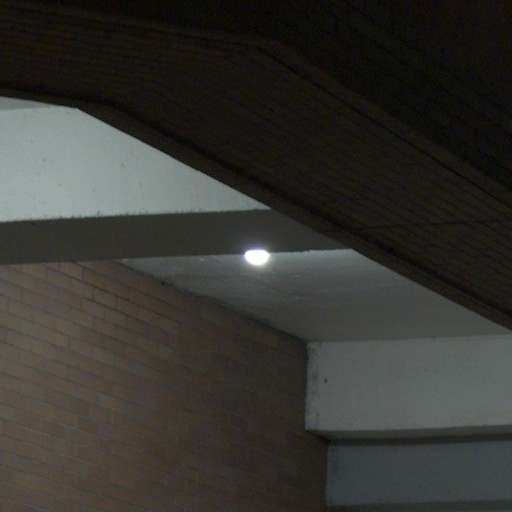}};
        \node[inner sep=0pt, right=0.05cm of fig32] (fig33) {\includegraphics[width=0.09\linewidth]{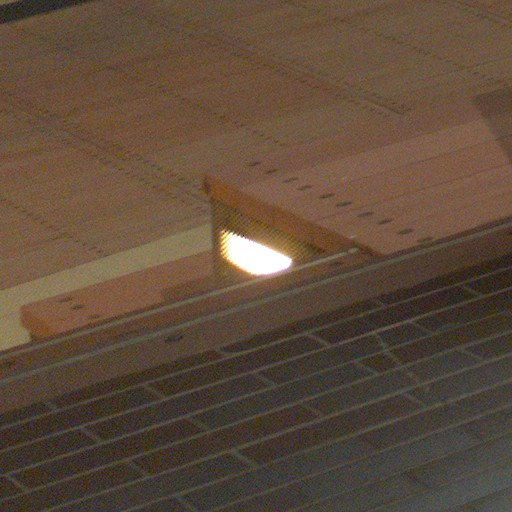}};
        \node[inner sep=0pt, right=0.05cm of fig33] (fig34) {\includegraphics[width=0.09\linewidth]{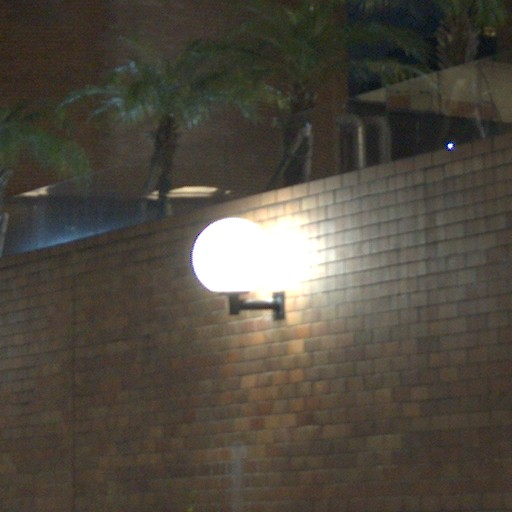}};
        \node[inner sep=0pt, right=0.05cm of fig34] (fig35) {\includegraphics[width=0.09\linewidth]{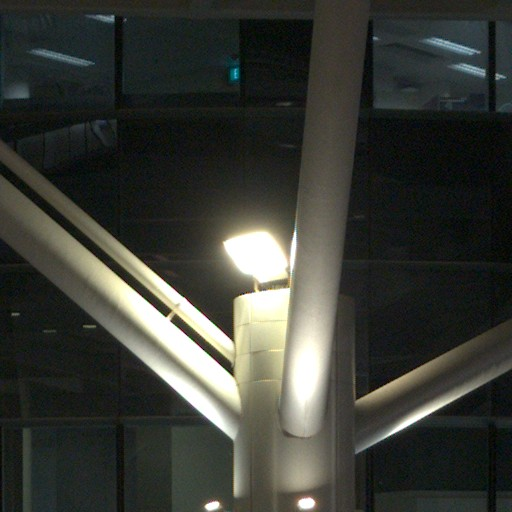}};
        \node[inner sep=0pt, right=0.15cm of fig35] (fig36) {\includegraphics[width=0.09\linewidth]{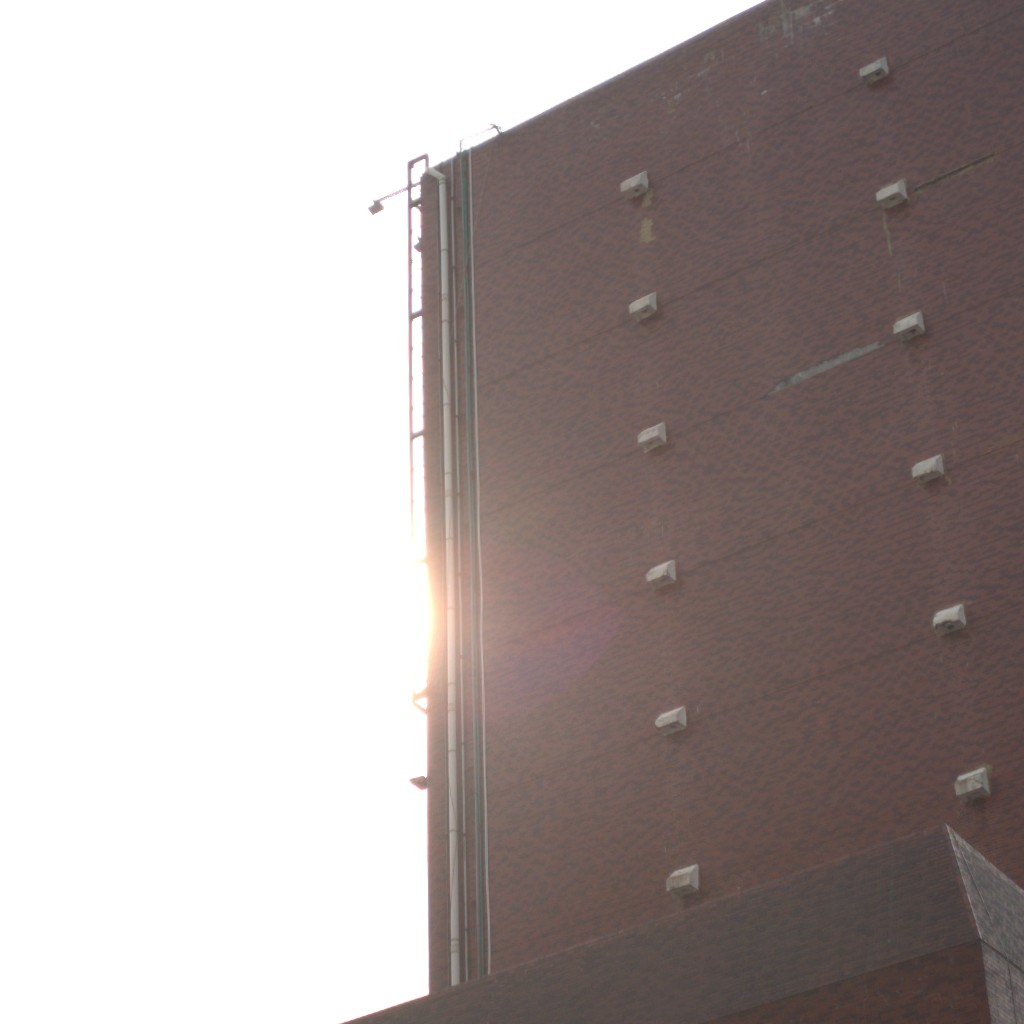}};
        \node[inner sep=0pt, right=0.05cm of fig36] (fig37) {\includegraphics[width=0.09\linewidth]{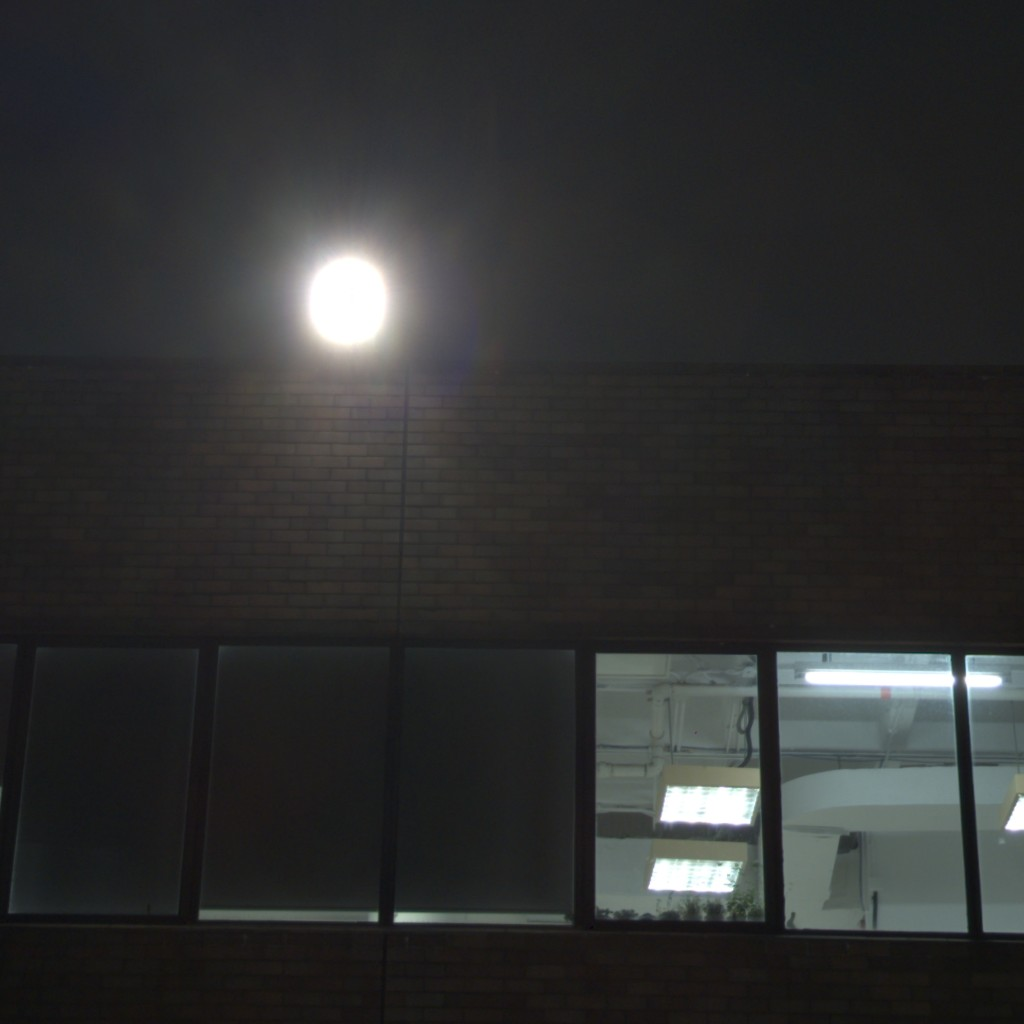}};
        \node[inner sep=0pt, right=0.05cm of fig37] (fig38) {\includegraphics[width=0.09\linewidth]{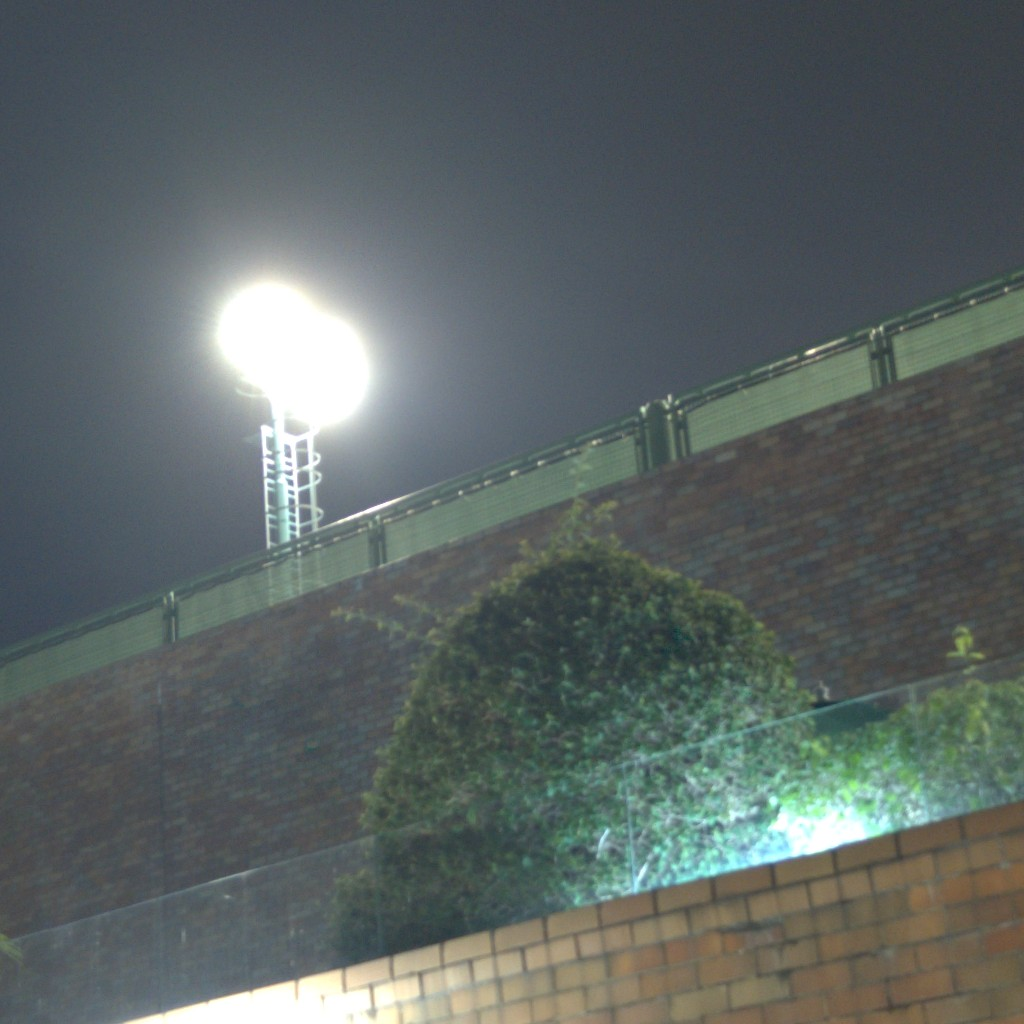}};
         \node[inner sep=0pt, right=0.05cm of fig38] (fig39) {\includegraphics[width=0.09\linewidth]{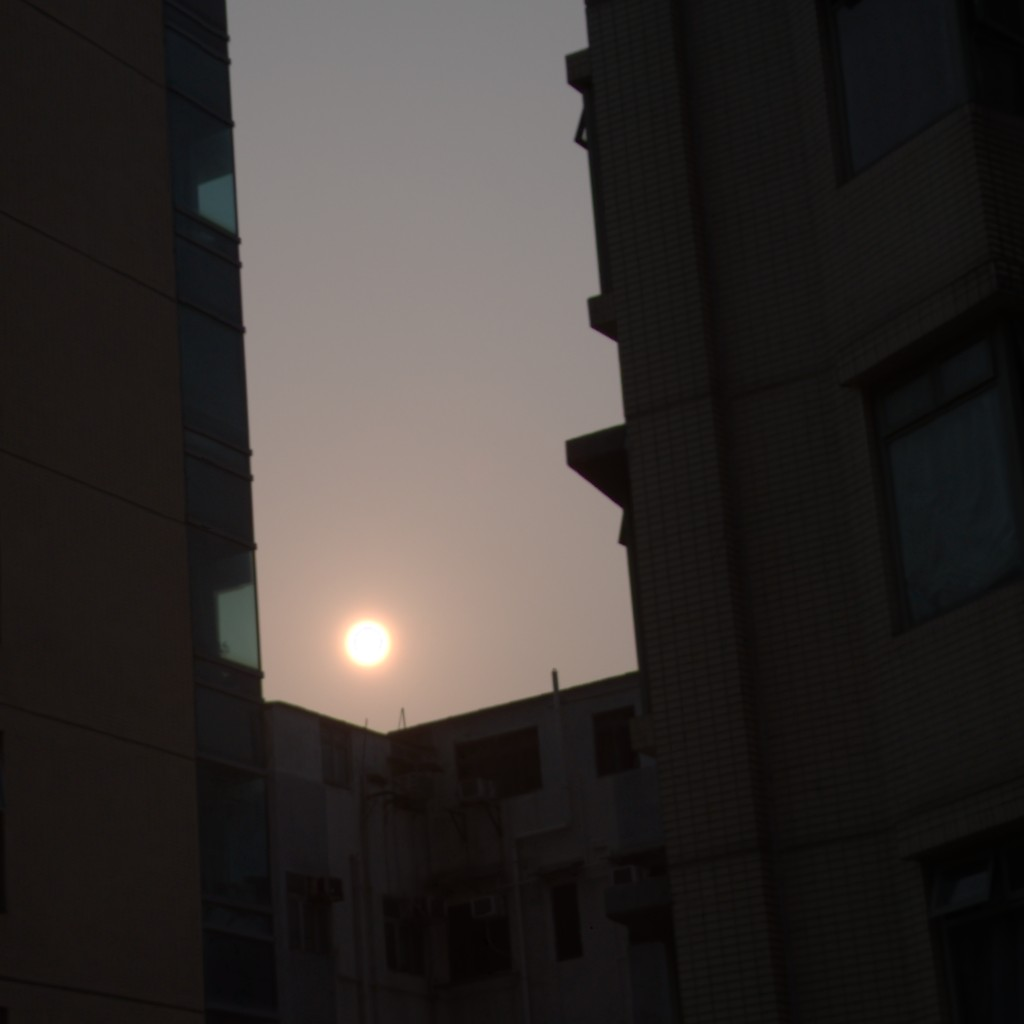}};
          \node[inner sep=0pt, right=0.05cm of fig39] (fig40) {\includegraphics[width=0.09\linewidth]{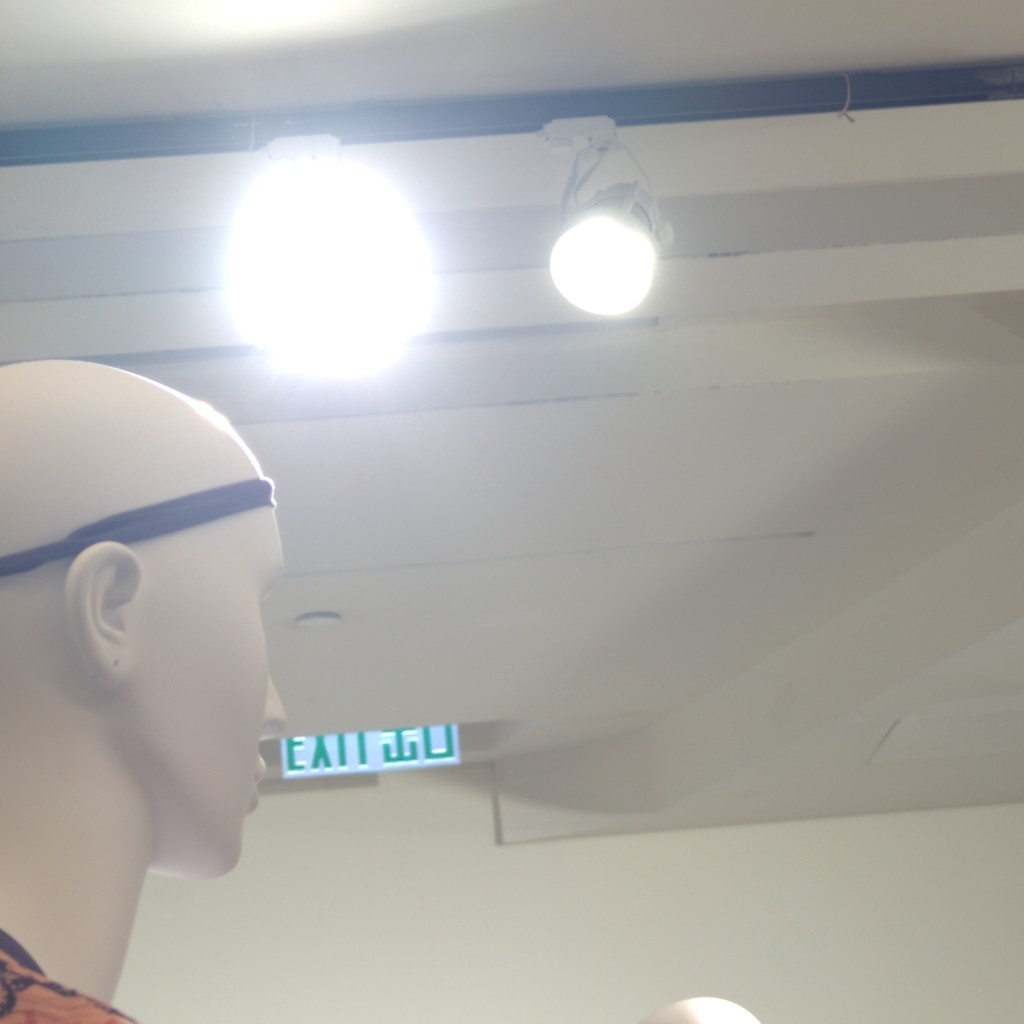}};
           % First row
         \node[inner sep=0pt, below=0.05cm of fig31] (fig41){\includegraphics[width=0.09\linewidth]{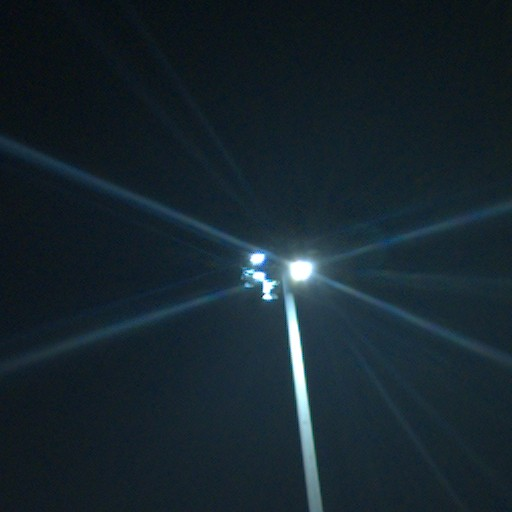}};
        \node[inner sep=0pt, right=0.05cm of fig41] (fig42) {\includegraphics[width=0.09\linewidth]{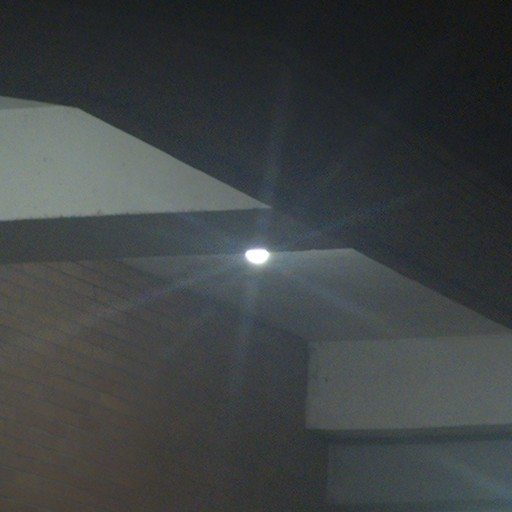}};
        \node[inner sep=0pt, right=0.05cm of fig42] (fig43) {\includegraphics[width=0.09\linewidth]{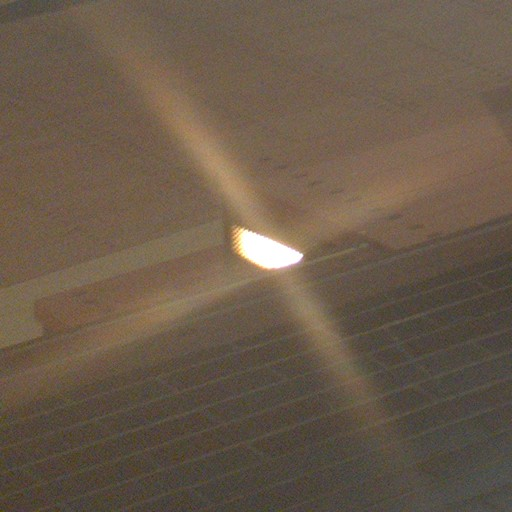}};
        \node[inner sep=0pt, right=0.05cm of fig43] (fig44) {\includegraphics[width=0.09\linewidth]{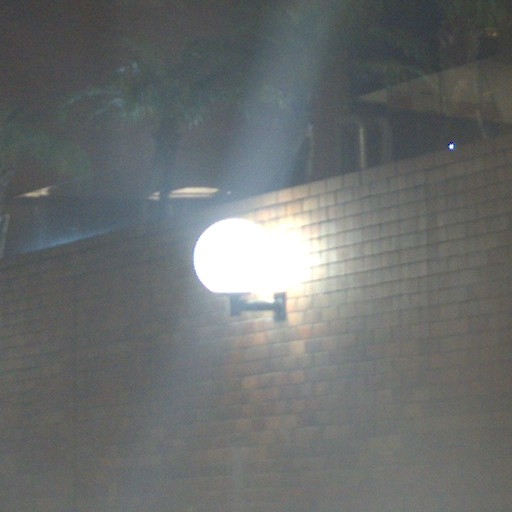}};
        \node[inner sep=0pt, right=0.05cm of fig44] (fig45) {\includegraphics[width=0.09\linewidth]{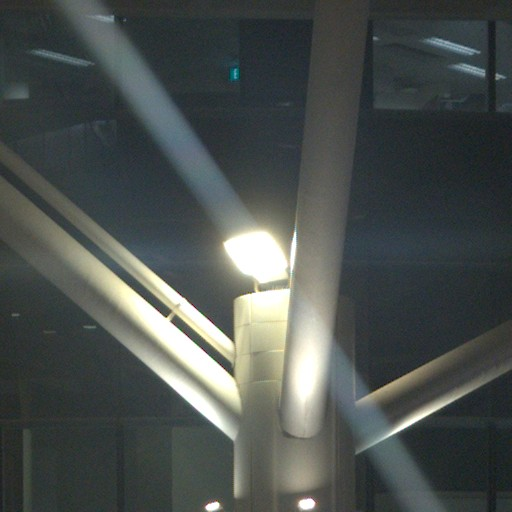}};
         \node[inner sep=0pt, right=0.15cm of fig45] (fig46) {\includegraphics[width=0.09\linewidth]{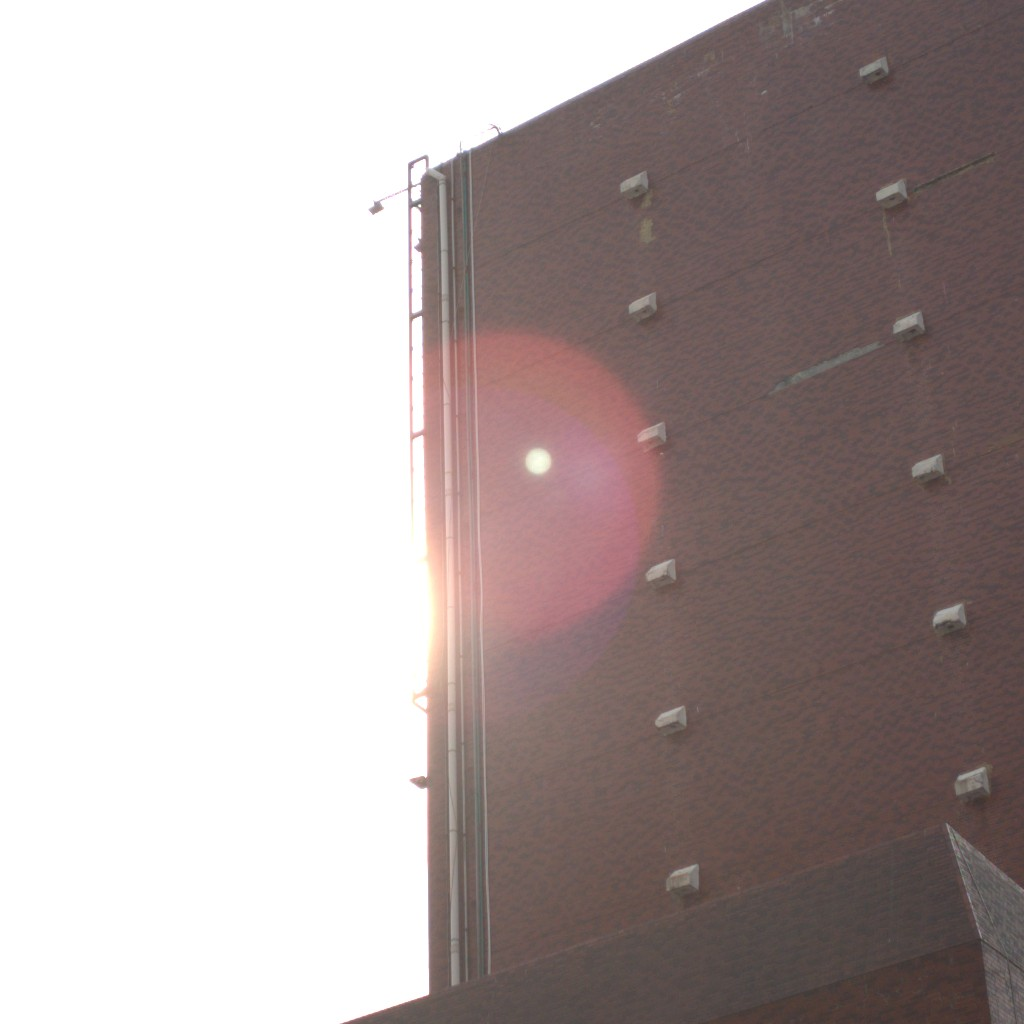}};
        \node[inner sep=0pt, right=0.05cm of fig46] (fig47) {\includegraphics[width=0.09\linewidth]{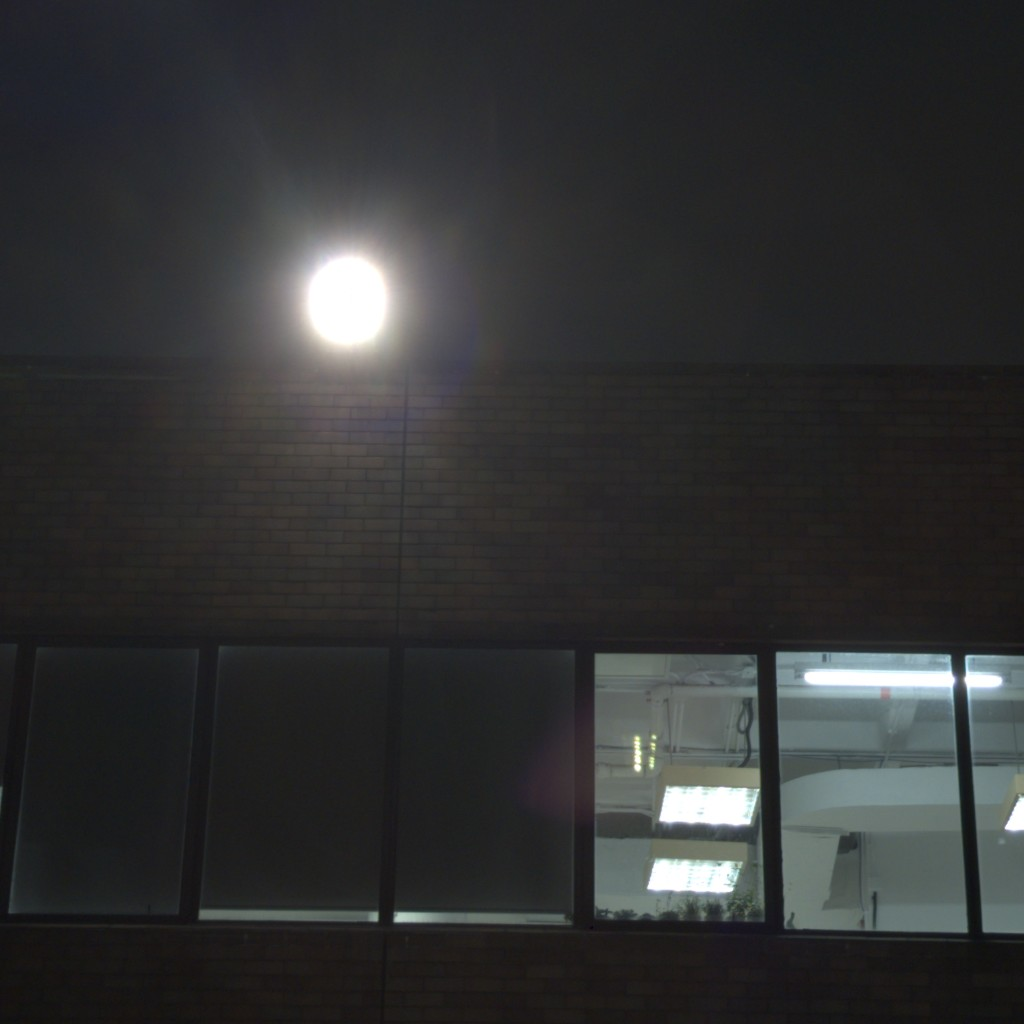}};
        \node[inner sep=0pt, right=0.05cm of fig47] (fig48) {\includegraphics[width=0.09\linewidth]{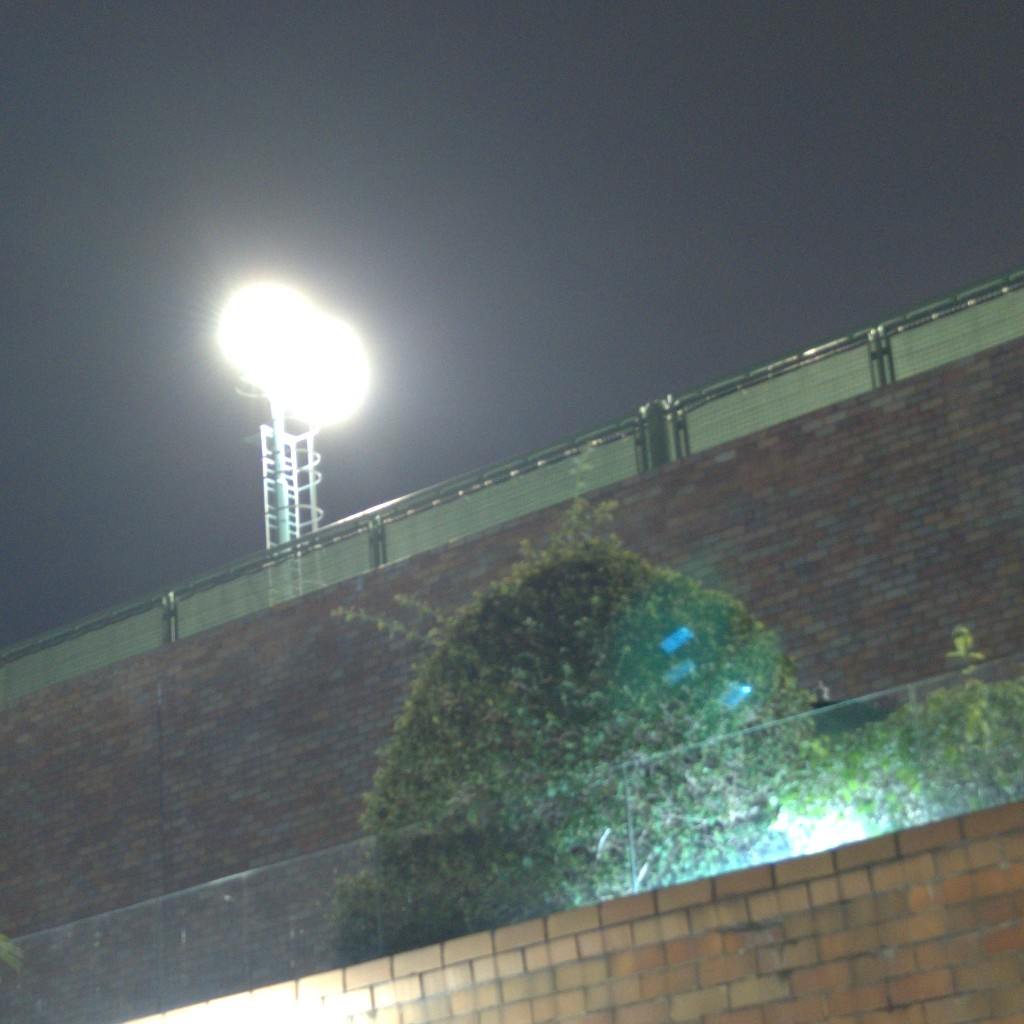}};
         \node[inner sep=0pt, right=0.05cm of fig48] (fig49) {\includegraphics[width=0.09\linewidth]{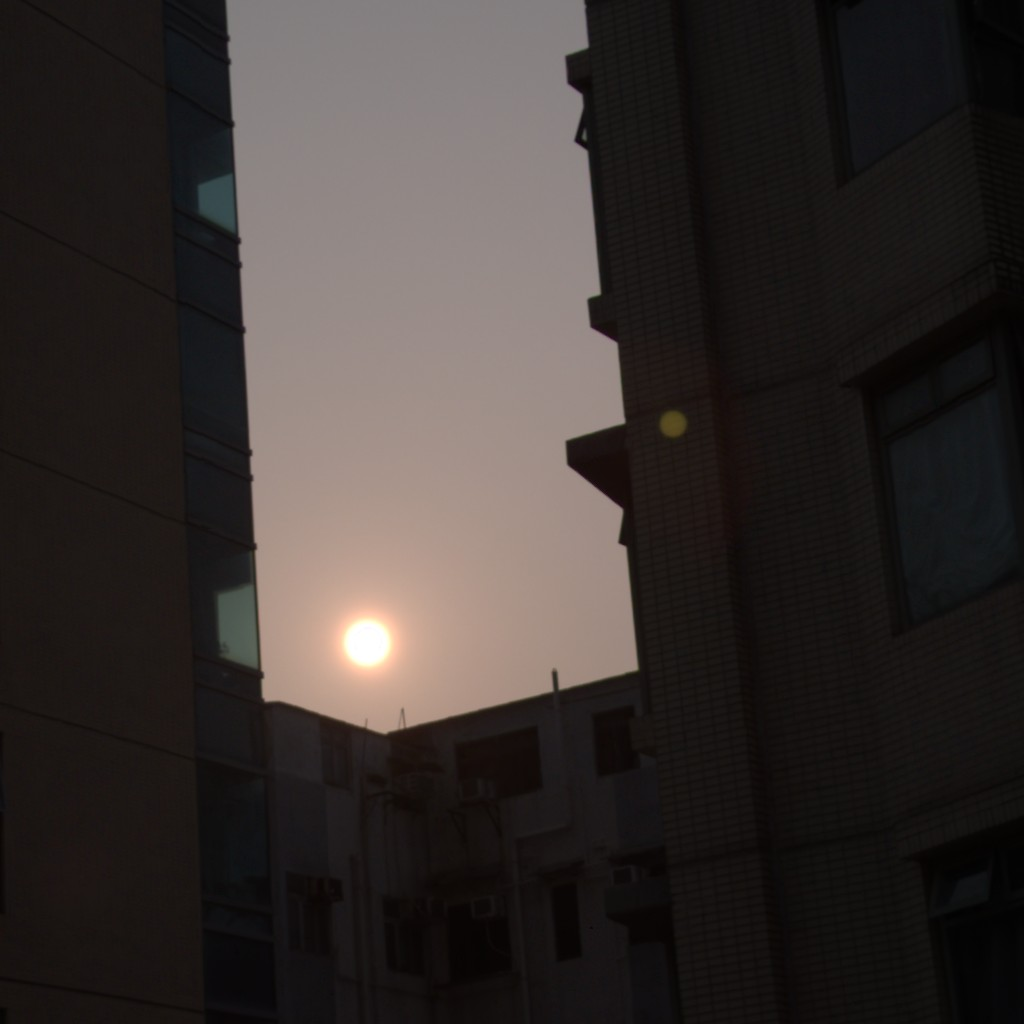}};
          \node[inner sep=0pt, right=0.05cm of fig49] (fig50) {\includegraphics[width=0.09\linewidth]{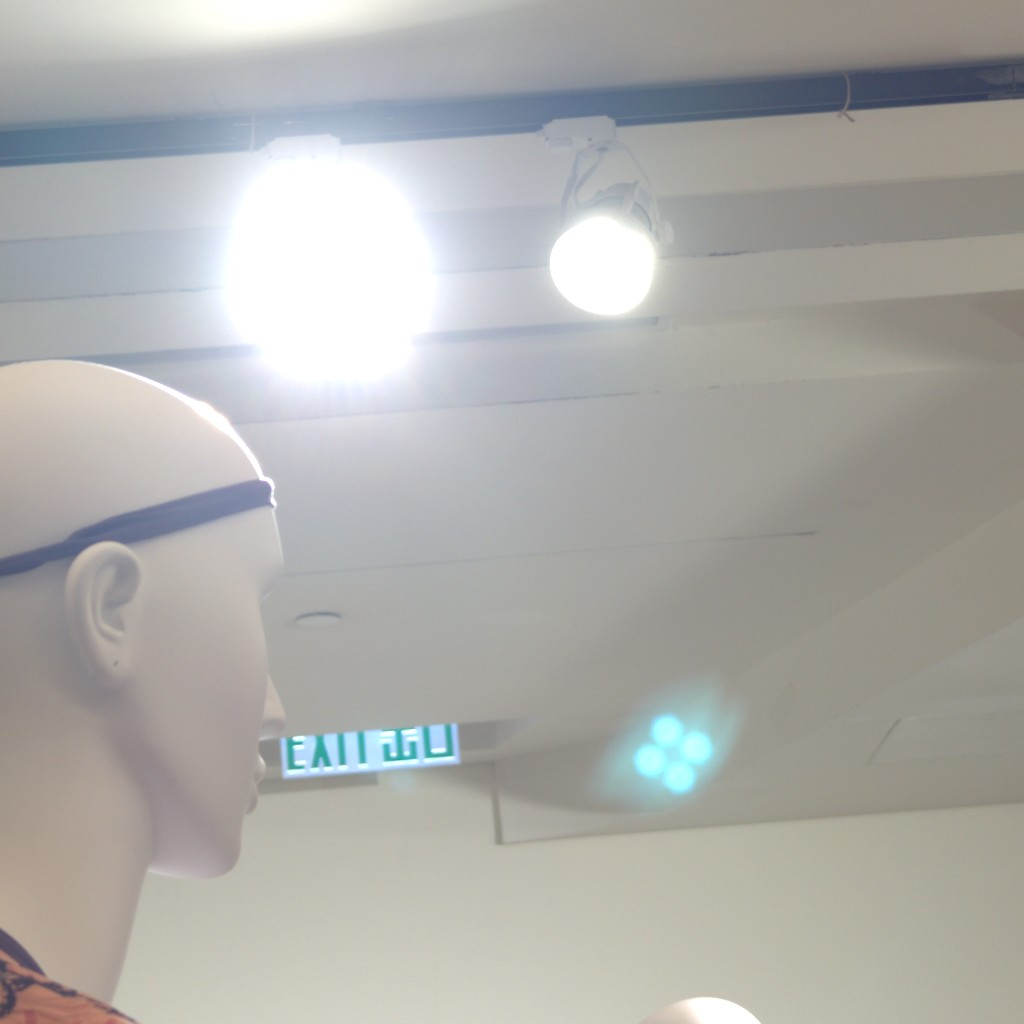}};
        % Second row
        \node[inner sep=0pt, below=0.05cm of fig41] (fig51) {\includegraphics[width=0.09\linewidth]{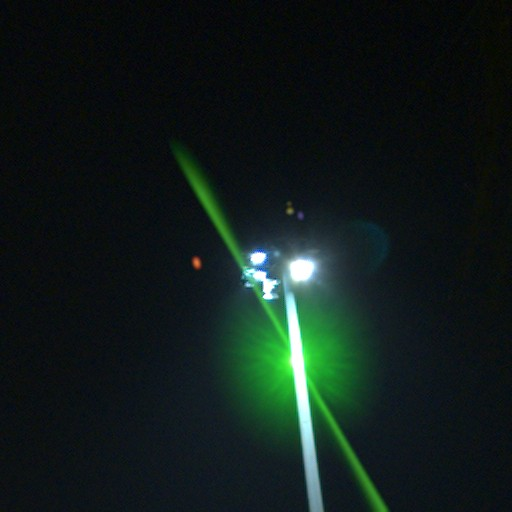}};
        \node[inner sep=0pt, right=0.05cm of fig51] (fig52) {\includegraphics[width=0.09\linewidth]{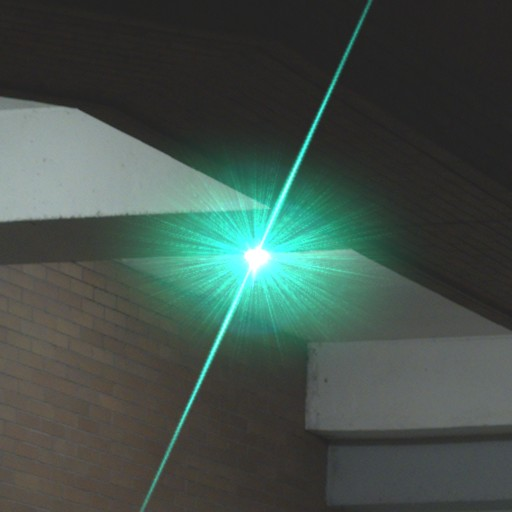}};
        \node[inner sep=0pt, right=0.05cm of fig52] (fig53) {\includegraphics[width=0.09\linewidth]{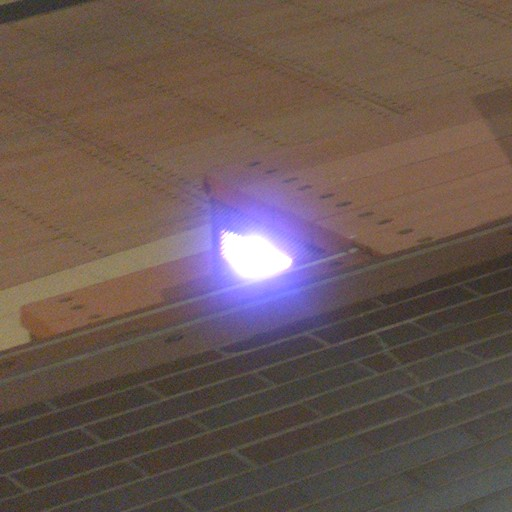}};
        \node[inner sep=0pt, right=0.05cm of fig53] (fig54) {\includegraphics[width=0.09\linewidth]{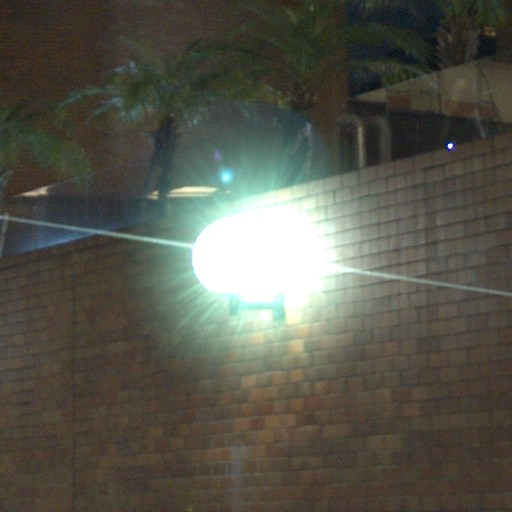}};
        \node[inner sep=0pt, right=0.05cm of fig54] (fig55) {\includegraphics[width=0.09\linewidth]{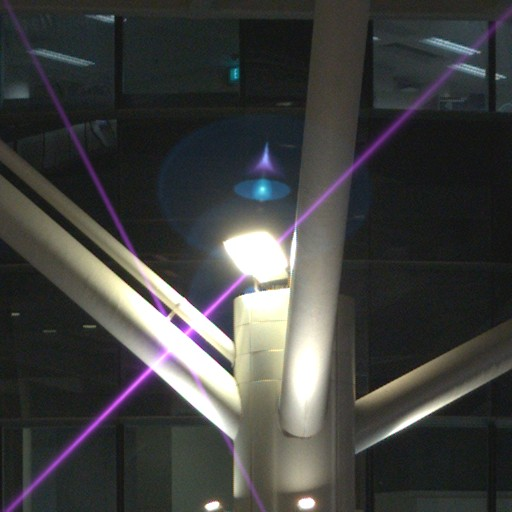}};
        \node[inner sep=0pt, right=0.15cm of fig55] (fig56) {\includegraphics[width=0.09\linewidth]{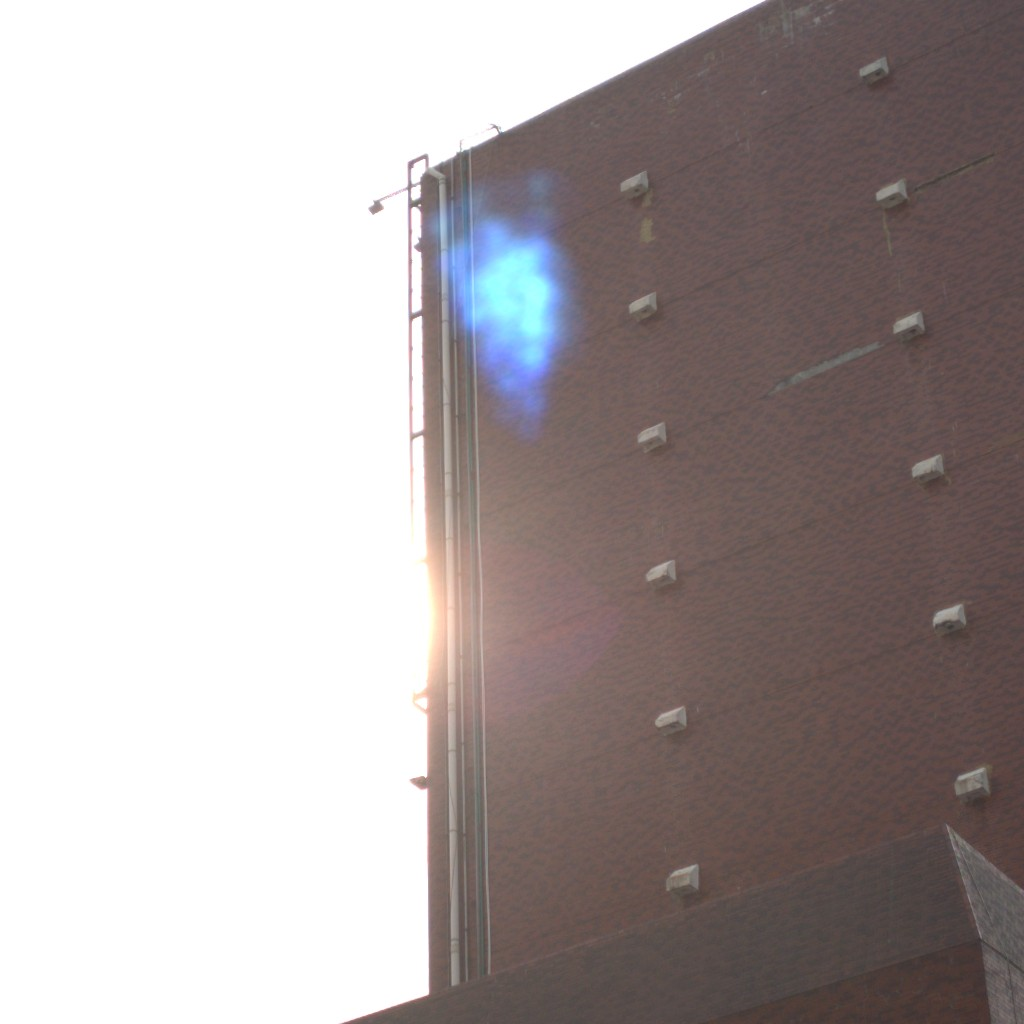}};
        \node[inner sep=0pt, right=0.05cm of fig56] (fig57) {\includegraphics[width=0.09\linewidth]{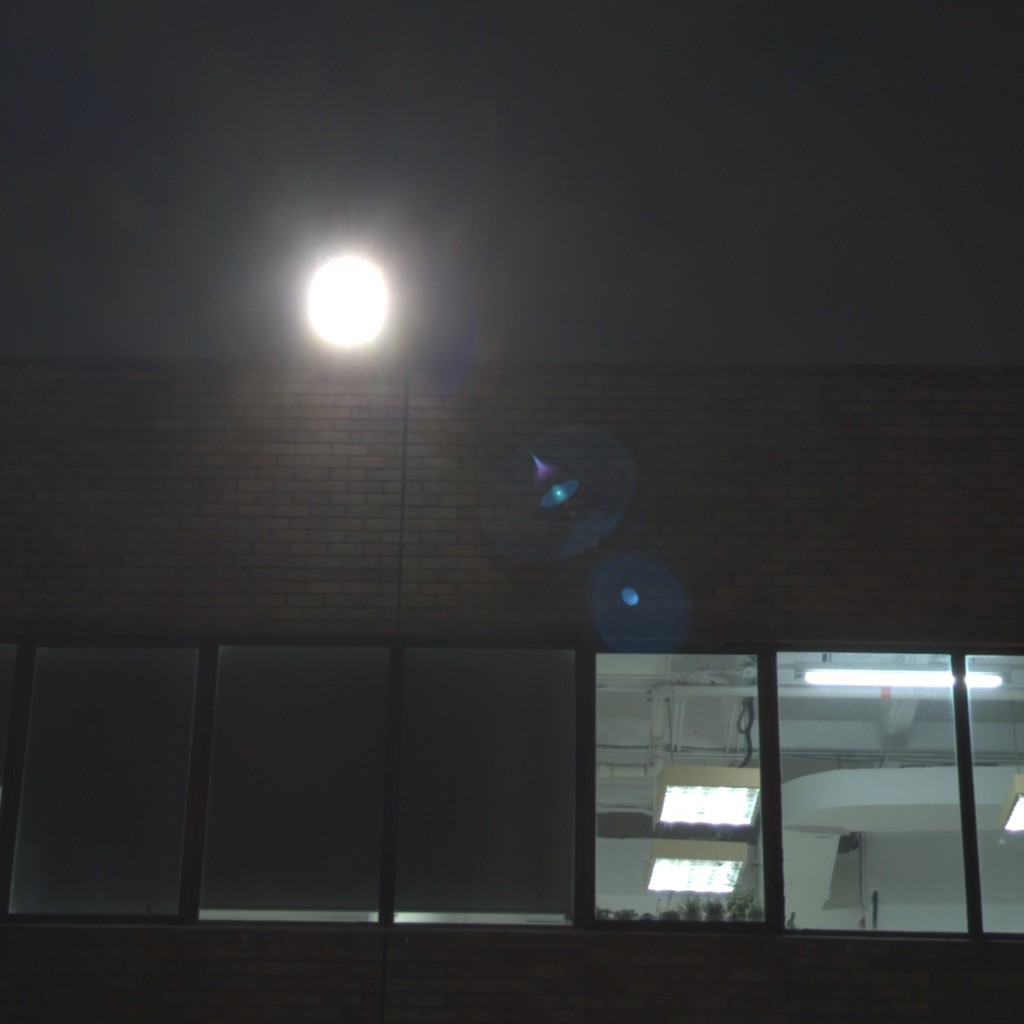}};
        \node[inner sep=0pt, right=0.05cm of fig57] (fig58) {\includegraphics[width=0.09\linewidth]{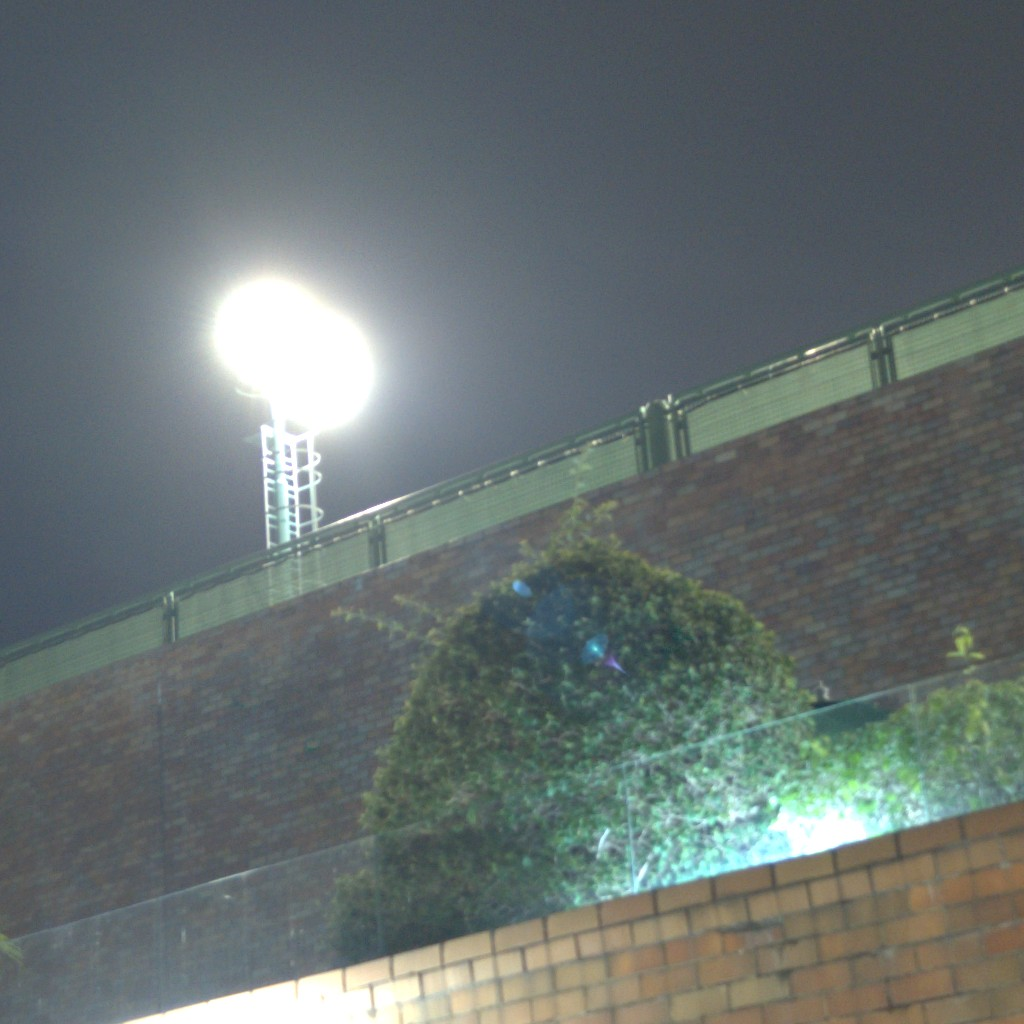}};
         \node[inner sep=0pt, right=0.05cm of fig58] (fig59) {\includegraphics[width=0.09\linewidth]{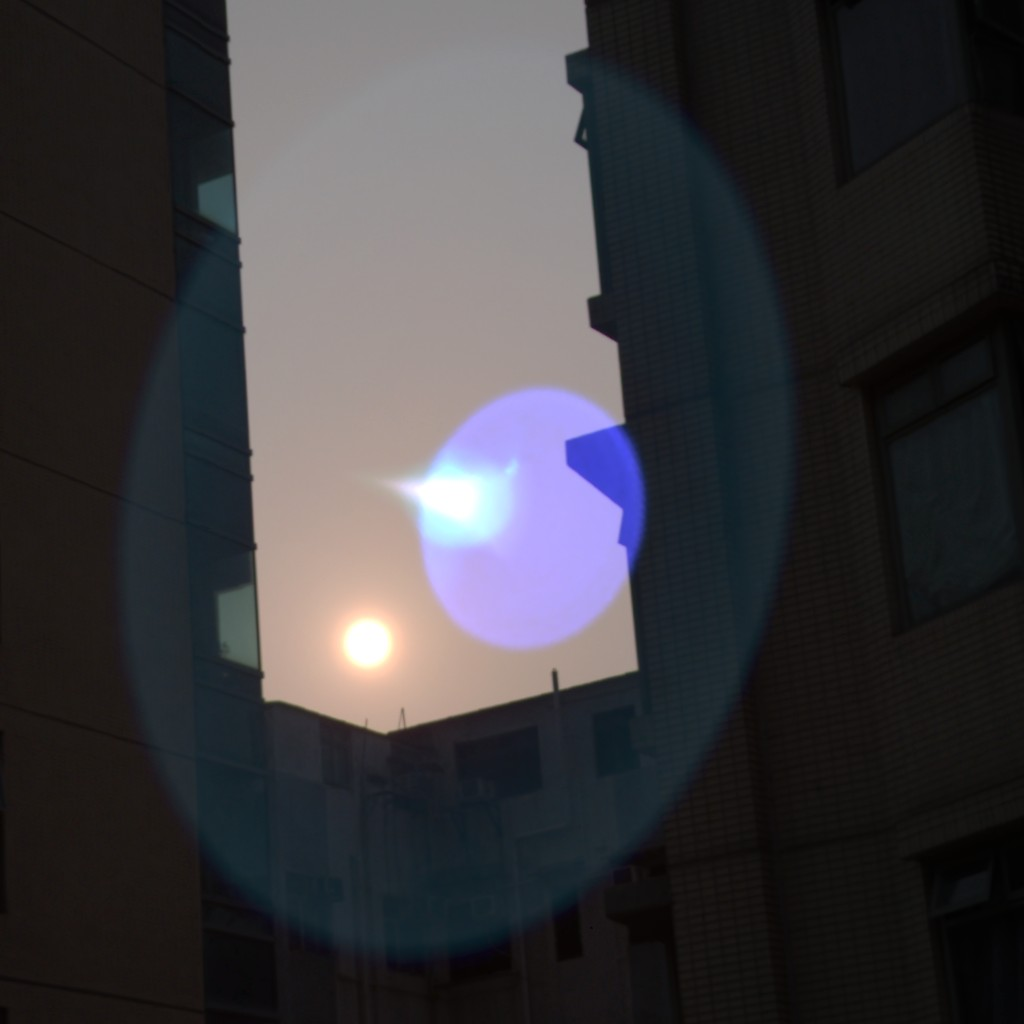}};
          \node[inner sep=0pt, right=0.05cm of fig59] (fig60) {\includegraphics[width=0.09\linewidth]{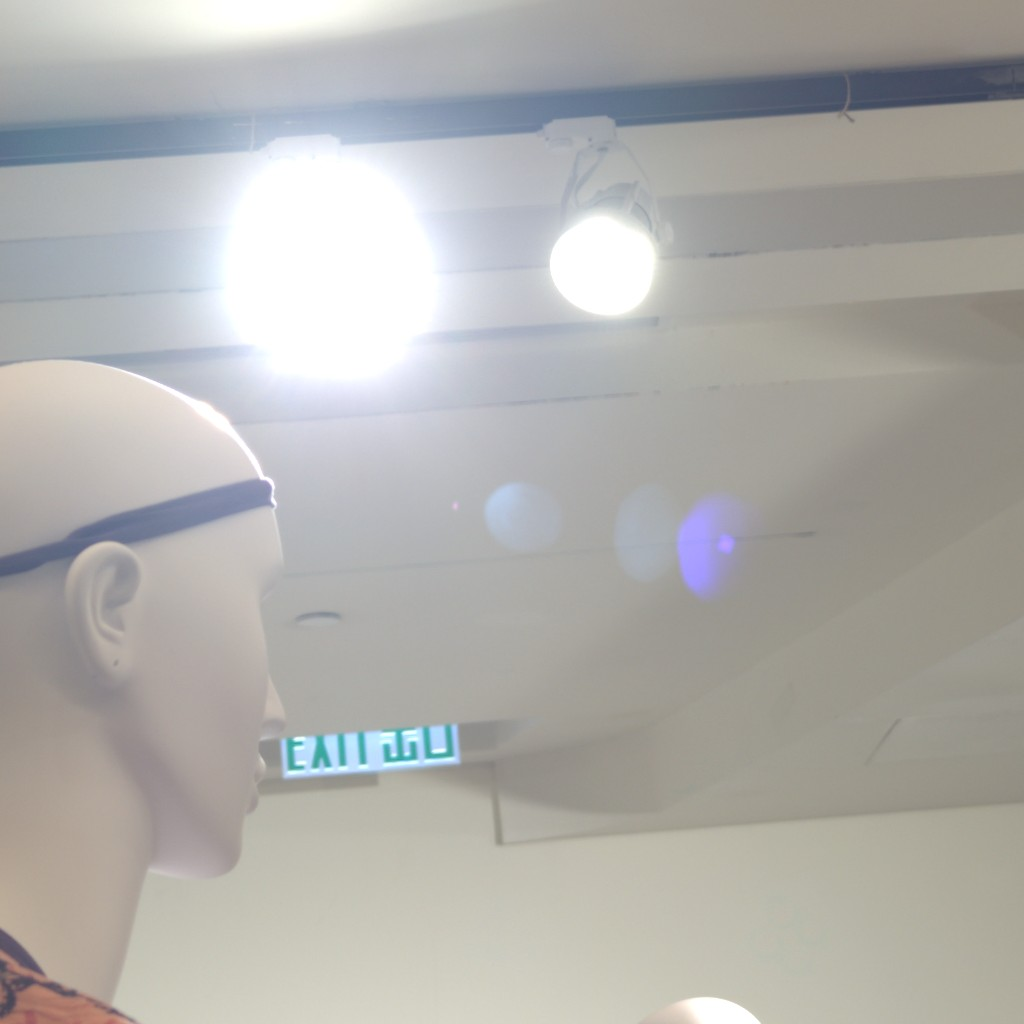}};
          
 \node[left=0.2cm of fig1, font=\fontsize{8}{12}\selectfont, rotate=90, anchor=center] {GT  (ours)};
        \node[left=0.2cm of fig31, font=\fontsize{8}{12}\selectfont, rotate=90, anchor=center] {GT (ours)};
        \node[left=0.2cm of fig11, font=\fontsize{8}{12}\selectfont, rotate=90, anchor=center] {ISPRGB (ours)};
        \node[left=0.2cm of fig41, font=\fontsize{8}{12}\selectfont, rotate=90, anchor=center] {RAW2RGB (ours)};
        \node[left=0.2cm of fig21, font=\fontsize{8}{12}\selectfont, rotate=90, anchor=center] {Flare7K};
        \node[left=0.2cm of fig51, font=\fontsize{8}{12}\selectfont, rotate=90, anchor=center] {Flare7K};
        \node[below=0.2cm of fig53, font=\fontsize{8}{12}\selectfont, anchor=center] {Scattering flare};
        \node[below=0.2cm of fig58, font=\fontsize{8}{12}\selectfont, anchor=center] {Reflective flare};
        
\draw[dashed] ([yshift=-0.075cm]fig21.south west) -- ([yshift=-0.075cm]fig30.south east);
\draw[dashed] ([xshift=0.075cm]fig5.north east) -- ([xshift=0.075cm]fig55.south east);
    \end{tikzpicture}
    % \caption{This figure provides examples showcasing the difference between real scattering and reflective flare images and synthesized images using Flare7k \cite{dai2022flare7k}. The first and the forth rows are the grountruth images from internal ISP and external processing piplines, respectively. The second and fifth rows are their corresponding flare-corrupted pairs. The third and last rows are the synthesized results generated with the groundtruth images using Flare7k.}
    \setlength{\belowcaptionskip}{-10pt}
 \caption{This figure presents examples that demonstrate the differences between real scattering and reflective flare images and their synthesized counterparts using Flare7K \cite{dai2022flare7k}. The first and fourth rows display the ground truth images obtained from the internal processing pipeline of mobile phones and external processing pipelines run on computers, respectively. The second and fifth rows depict the corresponding flare-corrupted pairs. The third and final rows showcase the synthesized results created using the ground truth images with Flare7K.}
 \label{fig: compare to Flare7k}
\end{figure*}

\section{Training Details}
Similar to Flare7K and Wu \etal \ , we use a U-Net for training as a baseline. The difference is that compared with their apporaches that segments light sources, perform flare removal and image blending to merge
the results back into the segmented images, we did not use such a blending approach because we notice that it may lead to inaccurate classification on flare and also worse performance in restoration quality. Instead, we use a U-Net for predict the flare area and substract it from the input for predicting a flare-free image.

\section{Visual Comparison on Data Generation}
In this section, we provide more visual comparison between our real image dataset and the synthetic datasdet from Flare7K
\input{visualdatageneration}
\section{Visual Comparison from Experiment}

% \section{Research Methods}

% \subsection{Part One}

% Lorem ipsum dolor sit amet, consectetur adipiscing elit. Morbi
% malesuada, quam in pulvinar varius, metus nunc fermentum urna, id
% sollicitudin purus odio sit amet enim. Aliquam ullamcorper eu ipsum
% vel mollis. Curabitur quis dictum nisl. Phasellus vel semper risus, et
% lacinia dolor. Integer ultricies commodo sem nec semper.

% \subsection{Part Two}

% Etiam commodo feugiat nisl pulvinar pellentesque. Etiam auctor sodales
% ligula, non varius nibh pulvinar semper. Suspendisse nec lectus non
% ipsum convallis congue hendrerit vitae sapien. Donec at laoreet
% eros. Vivamus non purus placerat, scelerisque diam eu, cursus
% ante. Etiam aliquam tortor auctor efficitur mattis.

% \section{Online Resources}

% Nam id fermentum dui. Suspendisse sagittis tortor a nulla mollis, in
% pulvinar ex pretium. Sed interdum orci quis metus euismod, et sagittis
% enim maximus. Vestibulum gravida massa ut felis suscipit
% congue. Quisque mattis elit a risus ultrices commodo venenatis eget
% dui. Etiam sagittis eleifend elementum.

% Nam interdum magna at lectus dignissim, ac dignissim lorem
% rhoncus. Maecenas eu arcu ac neque placerat aliquam. Nunc pulvinar
% massa et mattis lacinia.
